# Supplementary material for: Principles for sensitive and robust biomolecular interaction analysis - The limits of detection and resolution of diffraction-limited focal molography
Source: arXiv:1808.07956 ancillary file (2018-08-27)
Supplement: Supplementary file 1 [file Supplemental_Material.pdf]

# Supplemental Material

Andreas Frutiger,[1,*] Yves Blickenstorfer,[1,*] Silvio Bischof,[1] Csaba Forró,[1]
Matthias Lauer,[2] Volker Gatterdam,[1] Christof Fattinger,[2,†] and János Vörös[1,‡]
[1] *Laboratory of Biosensors and Bioelectronics, Institute of Biomedical Engineering, ETH Zürich, 8092 Zürich, Switzerland*
[2] *Roche Pharma Research and Early Development,*
*Roche Innovation Center Basel, 4070 Basel, Switzerland*
(Dated: August 23, 2018)

PACS numbers:

## I. DEFINITIONS

Here we list a few definitions related to analyte mass that are used in the manuscript. Focal molography detects the diffracted signal of a coherent ensemble of biomolecules. Nevertheless, the exact arrangement of the analyte mass on the ridges and grooves influences the diffraction efficiency of the molecular hologram and needs to be taken into account to formulate a limit of detection. For instance, a sinusoidal affinity modulation will require more mass bound to it than a canonical affinity modulation to produce the same molographic signal. As the diffraction efficiency compares different grating structures [1] a similar figure of merit - the analyte efficiency - can be defined for diffractometric biosensors. To obtain this, we first outline the definitions that are required to formulate the concept of the analyte efficiency of a particular affinity modulation.

**Affinity modulation:** The affinity modulation defines the functional distribution of the binding affinity across one groove and ridge after common offset [minimum value on the grooves] subtraction. This determines the mass modulation and hence the refractive index modulation after molecular recognition. Different ideal affinity modulations [δ-distributed, sinosoidal, canonical] are shown in Fig. 10(a) and explained in more detail below.

**Total mass on the mologram:** The *total mass on the mologram* $m_{\mathrm{tot}}$ is the total mass that has bound to ridges and grooves.

**Mass of the modulation:** The *mass of the modulation* $m_{\mathrm{mod}}$ is the total mass on the mologram subtracted by the common mass up to the minimum value on the grooves.

**Equivalent coherent mass:** The *equivalent coherent mass* $m_{\mathrm{coh}}$ is the amount of mass that would need to be placed on the center of the ridges [δ-distribution] to obtain the same diffraction efficiency as a mass which for instance is distributed sinusoidally or canonically.

**Equivalent coherent surface mass density:** The *equivalent coherent surface mass density* $\Gamma_{\mathrm{coh}}$ is the equivalent coherent mass divided by the footprint of the mologram [Bragg area, grooves and ridges included].

$$\Gamma_{\mathrm{coh}} = \frac{m_{\mathrm{coh}}}{A_{\mathrm{mologram}}} \tag{15}$$

It is a measure of the sensitivity of molography but practically not meaningful, since a $\delta$-distributed affinity modulation would be required to obtain it [see discussion below]. More appropriate for resolution comparison is the molographic surface mass density.

**Molographic surface mass density:** The *molographic surface mass density* $\Gamma$ is defined as the mass of the modulation $m_{\mathrm{mod}}$ divided by the entire molographic footprint.

$$\Gamma = \frac{m_{\mathrm{mod}}}{A_{\mathrm{mologram}}} \tag{16}$$

In our eyes, it is the most appropriate measure to compare molography to surface plasmon resonance and other refractometric biosensors which detect mass adlayer changes.

**Analyte efficiency:** In general, the *analyte efficiency* $\eta_{[\mathrm{A}]}$ is the ratio between the equivalent coherent mass and the total mass $m_{\mathrm{tot}}$ that has bound to the affinity modulation. The analyte efficiency can be computed from:

$$\eta_{[\mathrm{A}]} = \frac{m_{\mathrm{coh}}}{m_{\mathrm{tot}}} = \frac{\int_0^\Lambda \sin\left(\frac{2\pi\cdot x}{\Lambda}\right) f(x)\,dx}{\int_0^\Lambda f(x)\,dx} \tag{17}$$

The sinusoid stems from coherent weighting and $f(x)$ is the average mass distribution function [averaged over all periods of the mologram], determined by the affinity distribution. The integration is performed over one representative period of the mologram $\Lambda$. In other words, it is the normalized Fourier coefficient of the spatial frequency of the mologram [To be fully precise, since the mologram composes of lines with different spatial frequencies this would be a weighted sum over all periods in reality]. The concept of the analyte efficiency incorporates also imperfections of the lithography process such

*A. Frutiger and Y. Blickenstorfer contributed equally to this work.
†Electronic address: christof.fattinger@roche.com
‡Electronic address: janos.voros@biomed.ee.ethz.ch

TABLE I: Analyte efficiency for different ideal affinity modulations

| Affinity modulation | $f(x) - C_G$ | $\eta_{mod[A]}$ |
|---|---|---|
| $\delta$-distributed on ridge centers | $\delta\left(x - \frac{\Lambda}{4}\right) m_{mod}$ | 1 |
| Sinusoidal [ideal] | $\frac{m_{mod}}{\Lambda} + \frac{m_{mod}}{\Lambda} \sin\left(\frac{2\pi\cdot x}{\Lambda}\right)$ | 0.5 |
| Canonical [ideal] | $\frac{2\cdot m_{mod}}{\Lambda} \quad 0 \leqslant x < \frac{\Lambda}{2}$ | $\frac{2}{\pi}$ |

as finite mask contrast and nonlinear activation functions of the brushed polymer. However, for the discussion of the detection limit and resolution it is more appropriate to use the analyte efficiency of the modulation, since the common offset is not measured by molography.

**Analyte efficiency of the modulation:** The *analyte efficiency of the modulation* $\eta_{mod[A]}$ is the ratio between the equivalent coherent mass and the mass of the modulation. It can be computed analogously to the analyte efficiency by simply subtracting the common offset $C_G$ defined by the lowest value on the grooves from the affinity/mass distribution function.

$$\eta_{mod[A]} = \frac{m_{coh}}{m_{mod}} = \frac{\int_0^\Lambda \sin\left(\frac{2\pi\cdot x}{\Lambda}\right)\left(f(x) - C_G\right) dx}{\int_0^\Lambda \left(f(x) - C_G\right) dx} \tag{18}$$

Tab. I summarizes the analyte efficiency of the modulation of important affinity modulations in molography and Fig. 10(a) depicts them.

*$\delta$-distributed affinity modulation:* The $\delta$-distributed affinity modulation binds all mass to the very center of the ridges. The analyte efficiency of this structure is 1. However, it is not practically feasible for two reasons: First and most importantly, as the width of the activated region on the ridges approaches zero also the amount of available receptors does so. If not enough receptors are there to capture the analyte, the biosensor is rendered useless [2]. Second, to fabricate such small feature sizes is not trivial with current lithographic technologies.

*Sinusoidal affinity modulation:* The sinusoidal affinity modulation is obtained by phase mask lithography [interferometric exposure] under the assumption of a linear deprotection rate of the photoprotective group. To a first approximation the affinity modulation of the molograms in this contribution is sinusoidal. The analyte efficiency is 50 %, because a considerable amount of mass binds to the grooves and therefore cancels some of the mass on the ridges.

*Canonical affinity modulation:* The canonical affinity modulation is the one used in the original coupled mode theory equations of Fattinger and Tamir [3, 4]. The analyte efficiency of this modulation is slightly higher [63.6 %] but not fabricatable by phase mask lithography. Hence, the canonical mologram is only 1.3 [$\frac{4}{\pi}$] times better in terms of analyte efficiency than the sinusoidal mologram.

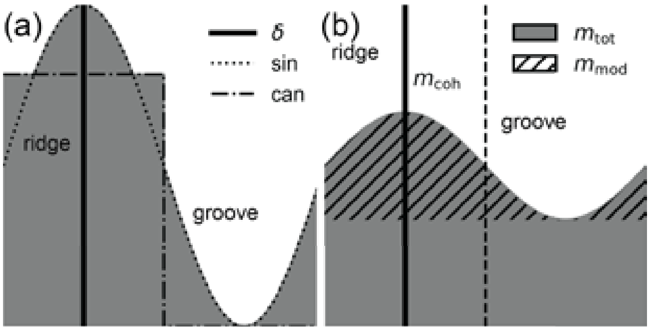


FIG. 10: Affinity modulations and different mass definitions (a) $\delta$-distributed, sinusoidal and canonical affinity modulation on the mologram. The canonical and sinusoidal are scaled such that the resulting mass modulations would have the same diffraction efficiency. (b) Definition of the total mass $m_{tot}$, the mass of the modulation $m_{mod}$ and the equivalent coherent mass $m_{coh}$

**Surface mass density modulation:** In the SI of a previous manuscript [5], we introduced the definition of the surface mass density modulation as the difference in mass density between ridges and grooves $\Delta_\Gamma = \Gamma_+ - \Gamma_-$. This definition was not precise in the way that we did not specify $\Gamma_+$ and $\Gamma_-$ unambiguously. Here we refine it in the following way: The mass density modulation is referred to as the mass of the modulation $m_{mod}$ divided by the area of the ridges $A_+$:

$$\Delta_\Gamma = \frac{m_{mod}}{A_+} \tag{19}$$

For a sinusoidal mass density modulation this corresponds to the peak-to-peak value $\Delta_{\Gamma_{PTP}} = \frac{m_{mod}}{A_+}$. For a canonical mologram, it corresponds to the difference in mass density between ridges and grooves $\Delta_{\Gamma_{can}}$. In addition, this definition is consistent for any mass distribution function.

## II. DESCRIPTION OF THE SIMULATION FRAMEWORK

The following section describes the Python simulation framework that calculates the scattered intensity in the focal spot from coherent protein particles.

### A. Waveguide and mologram calculation

The first step of the intensity calculation in the molographic spot is to solve the eigenvalue equations of the dielectric slab waveguide in order to determine the excitation field of the particles. This problem has been extensively investigated by Marcuse [6] in chapter 1.3 and

shall not be restated here. The framework allows to calculate the fundamental TE and TM modes whereas only the TE mode was investigated in this publication. Once the mode effective index is known, the molographic pattern with a defined focal spot and numerical aperture can be generated.

### B. Mologram creation and particle placement

The center of the molographic lines are given by formula 4 in Fattinger [3] and implemented in this way in the simulation framework [with $\xi = 0$]. The molographic lines are hyperbolas. An intuitive understanding of the shape of the pattern can be obtained by recalling that the circles of a Fresnel zone plate become ellipses for tilted plane wave incidence and are finally rendered hyperbolic for large incidence angles.

Furthermore, the molographic structure is constrained by an outer circle and a central cutout [to avoid second order bragg reflection - approximated as two circles - in reality these are hyperbolas as well, but for molograms with an NA of 0.5 and below this approximation is sufficient]. To place the particles efficiently, we make use of the symmetry of the molographic structure with respect to the xz-plane and seed particles only on the upper half of the mologram and invert the y-coordinate with probability 0.5 for every particle after seeding them all. Every molographic line in the positive [upper] half-plane can be seen as a curve $[\vec{c}(x) = (x, f(x))]$ subsequent to the circular constraints mentioned above. However, in order to place the particles uniformly along the line, one cannot simply randomly seed x, since the curves move much faster in [x,y] space on certain intervals of x, depending on their gradient. Therefore, some regions would be more densely seeded than others. The solution is to sample the normalized arc-length [can also be viewed as a cumulative distribution function] uniformly, given by:

$$C(x) = \frac{\int\limits_0^x \sqrt{1 + (\partial_x y)^2} dx}{\int\limits_0^{x_0} \sqrt{1 + (\partial_x y)^2} dx} \tag{20}$$

$x_0$ is the extent of the molographic line in x. Then, one simply needs to compute $x = C^{-1}(y)$, which is most easily done by interpolation. $y$ is uniformly distributed on the interval [0,1]. Once placed on the center of the ridges, the particles need to be sinusoidally shifted in order to account for the sinusoidal affinity modulation as present from phase mask lithography.

In summary, the procedure is the following:

1. Compute the mololines as a matrix of x and y coordinates. Calculate their lengths so as to have a vector of arc lengths $[l_0, l_1, \ldots, \mathrm{l_n}]$. Normalize the cumulative arc length of this vector to 1. Multiply the normalized cumulative arc length vector with the number of particles to be placed on the mologram to determine the number of particles that are placed on any line $j$.

2. For a chosen particle to be placed on line $j$, which is discretized and a vector of normalized arc length generated, sample a uniform random number on [0,1]. Select the index of the normalized arc length vector for this line that contains the entry that is closest to the sampled number. Use this index in order to get the position $x, y$, where the particle should be placed, from the discretized line.

3. Calculate the width $\delta$ of the line and seed the particle sinusoidally [with inverse CDF $C^{-1}(y) = \frac{\arccos(1-2x)}{\pi}, C^{-1} : [0,1] \to [0,\pi]$] with respect to the middle of the line on an interval equivalent to the calculated ridge width.

Since no mass is seeded on the grooves in the framework, the mass density on the ridges needs to be adjusted to take into account the mass on the grooves that would cancel some of the mass density on the ridges. The average mass density on the ridges that needs to be seeded sinusoidally is.

$$\frac{\int\limits_0^\pi \Delta_{\Gamma_{\mathrm{PTP}}} \sin(x)\, dx}{\int\limits_0^\pi dx} = \frac{2}{\pi} \cdot \Delta_{\Gamma_{\mathrm{PTP}}} \tag{21}$$

This times the area of the ridges gives the total number of particles that must be seeded on the mologram. It was further verified that canonical and sinusoidal placement give the same intensity when the particle number is adjusted accordingly [data not shown].

### C. Model of scattering protein particles

Proteins can be modeled as dipole scatterers. This approximation is valid, since the particle radius of a typical protein is only 2.5 nm, which is well-below the Rayleigh limit [7]. To use the dipolar approximation the refractive index and the volume need to be calculated for the dry protein sphere as a function of the molecular mass of the protein. The refractive index of the dry protein sphere can either be calculated from tabulated refractive index data for amino acids [8] and using the procedure from Ref. [9] or via the refractive index increment of proteins in water [9, 10]. The refractive index increment $\frac{dn}{dc}$ for proteins in water is generally accepted to be 0.182 ml/g for red light and in the absence of solvation effects. This value for the refractive index increment is a good approximation for most proteins [3, 11]. For a detailed discussion on the refractive index increment see Ref. [9]. We chose the approach with the protein refractive index increment. The dry refractive index of a protein is amenable from

$$n_{\mathrm{P}} = n_{\mathrm{c}}\sqrt{\frac{3n_{\mathrm{c}} + 4\rho_{\mathrm{P}}\frac{dn}{dc}}{3n_{\mathrm{c}} - 2\rho_{\mathrm{P}}\frac{dn}{dc}}} \tag{22}$$

where the molecular weight dependent mass density of the protein $\rho_{\mathrm{P}}\,(M_{\mathrm{P}})$ was calculated as reported in Ref. [12]. For SAv [$M_{\mathrm{P}} = 52.8$kDa] we calculated and used a mass density of 1.413 g/ml and a refractive index value of 1.598 in the simulations [for both air and water]. The volume of the protein and from this its radius was calculated according to

$$V_{\mathrm{P}} = \frac{M_{\mathrm{P}}}{N_A \rho_{\mathrm{P}}} = \frac{M_{\mathrm{P}}}{N_A}\frac{2}{3}\frac{dn}{dc}\frac{n_{\mathrm{P}}^2 + 2n_{\mathrm{c}}^2}{n_{\mathrm{c}}\,(n_{\mathrm{P}}^2 - n_{\mathrm{c}}^2)} \tag{23}$$

with the Avogadro constant $N_A$. For SAv the radius amounted to 2.46 nm.

### D. Field calculation and dipole emission near planar interfaces

Dipole emission near planar interfaces was carefully investigated by Novotny and summarized in the book Principles of Nanooptics, Chapter 10 [13–15]. We briefly summarized the most important equations and steps.

The electric dipole moment of a single Rayleigh scatterer is given by

$$\vec{p} = \varepsilon_0 \varepsilon_{\mathrm{c}} \alpha \vec{E}_0 \tag{24}$$

with $\varepsilon_0$ being the vacuum permittivity and $\varepsilon_{\mathrm{c}}$ standing for the permittivity of the cover medium. In this equation $\alpha$ is the static polarizability of the protein. This is not to be confused with the attenuation constant for which the symbol $\alpha$ is used throughout the rest of this publication. The polarizibilty is defined as

$$\alpha = 4\pi a^3 \frac{\varepsilon_{\mathrm{P}} - \varepsilon_{\mathrm{c}}}{\varepsilon_{\mathrm{P}} + 2\varepsilon_{\mathrm{c}}} \tag{25}$$

with $a$ being the radius and $\varepsilon_{\mathrm{P}}$ standing for the permittivity of the protein sphere.

The electric field of a single dipole in the allowed region in the substrate can be computed from the dipole potentials [15].

$$\begin{aligned} \vec{E} &= \begin{bmatrix} E_\theta \\ E_\phi \end{bmatrix} \\ &= \frac{k_{\mathrm{c}}^2}{4\pi\varepsilon_0\varepsilon_{\mathrm{c}}}\frac{e^{ik_{\mathrm{s}}r}}{r} \\ &\quad \times \begin{bmatrix} (p_x\cos\phi + p_y\sin\phi)\cos\theta\Phi_{\mathrm{s}}^{(2)} - p_z\cos\theta\Phi_{\mathrm{s}}^{(1)} \\ -(p_x\sin\phi - p_y\cos\phi)\,\Phi_{\mathrm{s}}^{(3)} \end{bmatrix} \end{aligned} \tag{26}$$

and in cartesian coordinates.

$$\vec{E} = \begin{bmatrix} E_x \\ E_y \\ E_z \end{bmatrix} = \begin{bmatrix} \cos\theta\cos\phi & -\sin\phi \\ \cos\theta\sin\phi & \cos\phi \\ -\sin\theta & 0 \end{bmatrix} \begin{bmatrix} E_\theta \\ E_\phi \end{bmatrix} \tag{27}$$

$p_x$, $p_y$ and $p_z$ are the components of the dipole moment vector. A dipole excited by the TE mode of a waveguide is oriented along $p_x$ only and therefore the above equations can be simplified.

The dipole potentials for the substrate half-space were defined by Novotny and Hecht [15].

$$\Phi_{\mathrm{s}}^{(1)} = \frac{n_{\mathrm{s}}}{n_{\mathrm{c}}}\frac{\cos\theta}{\tilde{s}_z(\theta)} t^{(p)}(\theta) e^{ik_s(z_0\tilde{s}_z(\theta) + d\cos\theta)} \tag{28a}$$

$$\Phi_{\mathrm{s}}^{(2)} = \frac{n_{\mathrm{s}}}{n_{\mathrm{c}}} t^{(p)}(\theta) e^{ik_s(z_0\tilde{s}_z(\theta) + d\cos\theta)} \tag{28b}$$

$$\Phi_{\mathrm{s}}^{(3)} = \frac{\cos\theta}{\tilde{s}_z(\theta)} t^{(s)}(\theta) e^{ik_s(z_0\tilde{s}_z(\theta) + d\cos\theta)} \tag{28c}$$

Note: The second potential has a wrong sign in [15]. The authors confirmed this and the equations stated here are correct. The Fresnel's transmission coefficients for a two interface structure were derived by Lukosz [16].

$$t^{(p,s)} = \frac{t_{\mathrm{c,f}}^{(p,s)} t_{\mathrm{f,s}}^{(p,s)} \exp\left(ik_{z,\mathrm{f}}t_{\mathrm{f}}\right)}{1 + r_{\mathrm{c,f}}^{(p,s)} r_{\mathrm{f,s}}^{(p,s)} \exp\left(2ik_{z,\mathrm{f}}t_{\mathrm{f}}\right)} \tag{29}$$

With Fresnel's reflection and transmission coefficients for single interfaces defined as

$$t_{n,m}^{(s)}(\theta) = \frac{2k_{z,n}}{k_{z,n} + k_{z,m}} \tag{30a}$$

$$t_{n,m}^{(p)}(\theta) = \frac{2\varepsilon_m k_{z,n}}{\varepsilon_m k_{z,n} + \varepsilon_n k_{z,m}}\sqrt{\frac{\varepsilon_n}{\varepsilon_m}} \tag{30b}$$

$$r_{n,m}^{(s)}(\theta) = \frac{k_{z,n} - k_{z,m}}{k_{z,n} + k_{z,m}} \tag{30c}$$

$$r_{n,m}^{(p)}(\theta) = \frac{\varepsilon_m k_{z,n} - \varepsilon_n k_{z,m}}{\varepsilon_m k_{z,n} + \varepsilon_n k_{z,m}} \tag{30d}$$

The factor $\tilde{s}_z(\theta)$ is defined as

$$\tilde{s}_z(\theta) = \sqrt{\left(\frac{n_{\mathrm{c}}}{n_{\mathrm{s}}}\right)^2 - \sin^2\theta} \tag{31}$$

Finally, the total intensity in the molographic focal spot is then given by the coherent superposition of the scattered fields of individual dipoles.

$$I_{\mathrm{avg}} = \frac{1}{2}\sqrt{\frac{\varepsilon_0\varepsilon_s}{\mu_0}} \sum_{i=1}^{N_{\mathrm{P}}} \vec{E}_i\left(\vec{r} - \vec{r}_0\right) \cdot \sum_{i=1}^{N_{\mathrm{P}}} \vec{E}_i^*(\vec{r} - \vec{r}_0) \tag{32}$$

where $N_{\mathrm{P}}$ is the number of coherently assembled particles.

### E. Implementation

The aggregated scattered intensities are calculated on a finite plane [screen] at regular, discrete space intervals [pixels]. The computation consists of the coherent summation of the fields of independent Rayleigh scatterers according to Eq. (32) for each individual pixel. Therefore, we make use of the parallel computation power of Graphical Processing Units [GPU]. We used an NVIDIA GTX 1080 Ti card and programmed it with its dedicated CUDA language [7.5 toolkit version]. No additional library than those provided per default by the toolkit were used. The complex computation library was not used but the equations were broken down to their complex and imaginary parts and treated separately. Special care needs to be taken to use atomic additions when aggregating the fields on a given pixel. The low memory cost and the speedup provided by this approach allowed the computation of 231 million protein scatterers on a screen of 150 x 150 pixels in only 1650 seconds. A further speed up could be achieved by optimizing the memory traffic during the computation, for example by using shared memory and take advantage of thread warping.

## III. MOLOGRAPHIC SIGNAL INTENSITY FROM COUPLED MODE THEORY AND RAYLEIGH SCATTERING

The molographic signal [average intensity in the Airy disk] can be computed from coupled mode theory but also via summation of Rayleigh scatterers [neglecting the interface effects], which give basically the same result. Here we outline the procedure to arrive at these expressions. To obtain an expression of the intensity in the focal spot via coupled mode theory, we start from Eq. (6) in Fattinger . By using $\Lambda \approx \lambda/n_\mathrm{c}$ and substituting $\frac{\partial N}{\partial n_\mathrm{c}}$ with Eq. (7) in Fattinger [3] we get

$$P_\mathrm{diff} = 2\pi \frac{D^2}{\lambda^2}\left(\frac{dn}{dc}\right)^2 {\Delta_{\Gamma_\mathrm{can}}}^2 \frac{n_\mathrm{c}\left(n_\mathrm{f}^2 - N^2\right)}{N t_\mathrm{eff}\left(n_\mathrm{f}^2 - n_\mathrm{c}^2\right)} P_\mathrm{wg} \quad (33)$$

There are a few differences compared to the equation in Fattinger [3]. First, $P_\mathrm{diff}$ is the total power coupled out in Watts, whereas Fattinger defined it as a power per line $\left[\frac{\mathrm{W}}{\mathrm{m}}\right]$. We chose this definition because it is the total power that is then focused onto the Airy disk and not a power per line. We still keep the definition of $P_\mathrm{wg}$ as power per line $\left[\frac{\mathrm{W}}{\mathrm{m}}\right]$. $\Delta_{\Gamma_\mathrm{can}}$ denotes the canonical surface mass modulation. This definition is by a factor 2 higher than the original one used in Fattinger [3], which corresponds to the molographic surface mass density here. In order to determine the intensity in the focal spot, we realize that the diffracted power is distributed over the Airy disk. From the properties of the Bessel function of the first kind that describes the shape of the Airy disk, it follows that 83.8 % of the total diffracted power is contained within the first zeros of the Bessel function [17].

$$I_\mathrm{avg} = 0.838 \cdot \frac{P_\mathrm{diff}}{A_\mathrm{Airy}} \quad (34)$$

The area of the Airy disk is given by the readout wavelength and the numerical aperture of the system [18]

$$A_\mathrm{Airy} = 0.37\pi \frac{\lambda^2}{\mathrm{NA}^2} \quad (35)$$

with the approximative numerical aperture $\mathrm{NA} = \frac{D n_\mathrm{s}}{2f}$. Therefore, the average intensity on the Airy disk calculated via coupled mode theory reads

$$\begin{aligned} I_\mathrm{avg,CMT} &= 4.53 \cdot \mathrm{NA}^2 \frac{n_\mathrm{c} \cdot \left(n_\mathrm{f}^2 - N^2\right)}{t_\mathrm{eff} N \left(n_\mathrm{f}^2 - n_\mathrm{c}^2\right)} \left(\frac{dn}{dc}\right)^2 \\ &\times \frac{D^2}{\lambda^4} {\Delta_{\Gamma_\mathrm{can}}}^2 P_\mathrm{wg} \end{aligned} \quad (36)$$

To see the analogy to Rayleigh scattering, we rewrite the power in the waveguide as the intensity on the waveguide surface as

$$I_0 = \frac{n_c}{2Z_w} A^2 = n_c \frac{2\left(n_\mathrm{f}^2 - N^2\right)}{N t_\mathrm{eff}\left(n_\mathrm{f}^2 - n_\mathrm{c}^2\right)} P_\mathrm{wg} \quad (37)$$

and furthermore generalize the canonical surface mass density modulation with the analyte efficiency of the modulation $\eta_{\mathrm{mod}\,[\mathrm{A}]}$.

$$I_\mathrm{avg,CMT} = 5.59 \cdot \mathrm{NA}^2 \left(\frac{dn}{dc}\right)^2 \frac{D^2}{\lambda^4} {\eta_{\mathrm{mod}\,[\mathrm{A}]}}^2 {\Delta_\Gamma}^2 I_0 \quad (38)$$

The expression for Rayleigh scattering in plane-polarized light [7] can be easily obtained from Eq. (1) in Ref. [3].

$$I_\mathrm{Airy,max,RS} = 9\pi^2 \frac{n_\mathrm{c}^4}{f^2\lambda^4} \frac{1}{\rho_\mathrm{P}^2} \frac{M_\mathrm{P}^2 N_\mathrm{P}^2}{N_A^2} \frac{\left({n_\mathrm{P}}^2 - n_\mathrm{c}^2\right)^2}{\left(n_\mathrm{P}^2 + 2n_\mathrm{c}^2\right)^2} I_0 \quad (39)$$

Where we have replaced the volume of a single protein according to $V_\mathrm{P} = \frac{M_\mathrm{P}}{\rho_\mathrm{P} N_A}$ and generalized the expression to an ensemble of $N_\mathrm{P}$ coherent proteins. It has to be noted that Eq. (2) in Ref. [3] which is used to calculate the volume of the protein from the refractive index increment is an approximation. Eq. (23) should be used instead.

Eq. (39) describes the maximum intensity in the Airy disk and not yet the average intensity. The ratio between the maximum and the average can be readily calculated by integration over the Airy disk such that

$$I_{\mathrm{Airy}_\mathrm{max}} = \frac{\int_0^{3.83} r dr}{\int_0^{3.83} \left(\frac{2J_1(r)}{r}\right)^2 r dr} I_\mathrm{avg} = 4.378 \cdot I_\mathrm{avg} \quad (40)$$

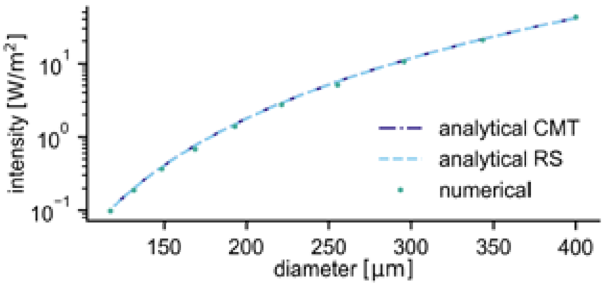


FIG. 11: Comparison of the different models in water to predict the average intensity in the Airy disk [simulation parameters were the same as the ones described in Fig. 5, which is in air]. One can see that the two analytical models nearly perfectly match the numerical calculations.

where $J_1$ is the Bessel function of the first kind. Inserting Eq. (39) for $I_{\mathrm{Airy}_{\max}}$ yields

$$I_{\mathrm{avg,RS}} = 2.056 \cdot \pi^2 \frac{n_c^4}{f^2\lambda^4} \frac{1}{\rho_P^2} \frac{M_P^2 N_P^2}{N_A^2} \frac{\left(n_P^2 - n_c^2\right)^2}{\left(n_P^2 + 2n_c^2\right)^2} I_0 \quad (41)$$

Using the definitions for the numerical aperture $\mathrm{NA} = \frac{n_c D}{2f}$ and the conversion from protein number to surface mass density modulation $\frac{M_P^2 N_P^2}{N_A^2} = \frac{D^4\pi^2}{64} {\eta_{\mathrm{mod\,[A]}}}^2 {\Delta_\Gamma}^2$ results in

$$I_{\mathrm{avg,RS}} = 1.268 \cdot \pi^2 n_c^2 \frac{\left(n_P^2 - n_c^2\right)^2}{\left(n_P^2 + 2n_c^2\right)^2} \mathrm{NA}^2 \times \frac{1}{\rho_P^2} \frac{D^2}{\lambda^4} {\eta_{\mathrm{mod\,[A]}}}^2 {\Delta_\Gamma}^2 I_0 \quad (42)$$

And finally with the definition of the refractive index increment for proteins [Eq. (4)] one obtains

$$I_{\mathrm{avg,RS}} = 5.56 \cdot \mathrm{NA}^2 \left(\frac{dn}{dc}\right)^2 \frac{D^2}{\lambda^4} {\eta_{\mathrm{mod\,[A]}}}^2 {\Delta_\Gamma}^2 I_0 \quad (43)$$

which is beside a small numerical error the same as the expression from coupled mode theory [Eq. (38)].

Measurements in air are an unusual case in label-free investigations and were only chosen here for the sake of experimental simplicity. In the practical settings, namely in water, both of these models nearly perfectly coincide with the numerical computations that takes the interfaces into account [Fig.(11)].

## IV. DEPHASING AS A LIMITATION ON MOLOGRAM SIZE

As described in the main manuscript we expect the amount of sample volume to limit the mologram size for diameters > 1 mm. However, it is already non-trivial to achieve diffraction-limited focusing for molograms up to 400 μm diameter on high refractive index waveguides, since gradients in effective refractive index can also result in a limitation on mologram size. The most prominent source for a gradient in effective index stems from the wedgedness of the waveguide [see Fig. 12(c)]. Due to the bell-shaped deposition curve of most sputtering systems used in research [19] or due to the thickness gradients introduced by the coating process in Sol-Gel waveguide fabrication methods [spin coating] [20], the resulting waveguides exhibit a certain degree of wedging. For sputtering fabrication, this is less of a problem if the deposition is performed by industrial scale large area sputtering systems. The wedging of the waveguide introduces a gradient in effective refractive index. This leads to an accumulated phase mismatch between the synthetic hologram [designed for constant effective refractive index] and the guided mode. After a certain propagation distance, which we call the dephasing length, light scattered at the first and the last line of the mologram interferes destructively [see Fig.12].

We can use coupled mode theory to address the effect of dephasing on the diffracted power. For simplicity, we model the mologram as a sinusoidal grating with a constant period. We start from Eqs. (3.4-8) (3.4-10) and (5.2-1) in Marcuse [6]. However, we adapt these expressions for the case of a guided mode with a non-constant phase.

$$P_{\mathrm{diff}} = \left\langle |c|^2 \right\rangle \propto \left\langle \left| \int_0^D f(z) e^{i((\beta_{\mathrm{in}} - \beta_{\mathrm{out}})z + \phi(z))} dz \right|^2 \right\rangle \quad (44)$$

with $f(z) = \sin \frac{2\pi}{\Lambda} z = e^{-i\frac{2\pi}{\Lambda}z}$ being the grating function of a sinusoidal grating. For a constant effective refractive index gradient the accumulated phase mismatch reads

$$\phi(z) = -\int_0^z k_0 \frac{dN}{dz} z' dz' = -k_0 \frac{dN}{dz} \frac{z^2}{2} \quad (45)$$

We assume the detuning parameter $d = \beta_{\mathrm{in}} - \beta_{\mathrm{out}} - \frac{2\pi}{\Lambda}$ over the entire waveguide to be constant. Then we can write

$$P_{\mathrm{diff}} \propto \left\langle \left| \int_0^D e^{idz - isz^2} dz \right|^2 \right\rangle \quad (46)$$

Where $s = -\frac{k_0}{2} \frac{dN}{dz}$ is the dephasing parameter. After integration and multiplying with the complex conjugate we obtain.

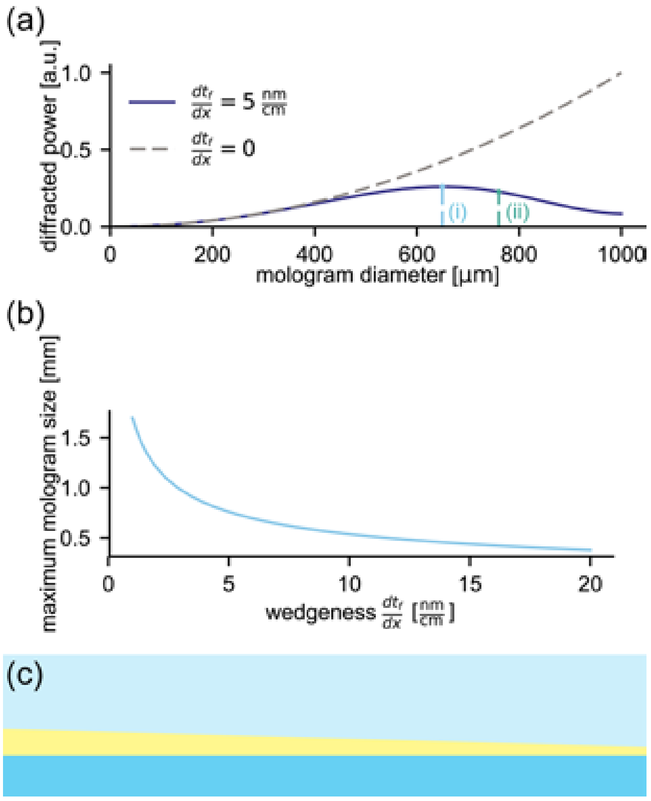


FIG. 12: (a) Diffracted power of a sinusoidal grating as a function of mologram size for a waveguide with no effective index gradient [grey] and with a wedgedness of 5 nm/cm (i) maximum reasonable mologam size (ii) dephasing length (b) maximum mologram size for different waveguide wedgedness. The calculations were performed for $n_\mathrm{f} = 2.117$, $n_\mathrm{c} = 1$, $n_\mathrm{s} = 1.521$ and $\lambda = 632.8$ nm (c) illustration of a waveguide with a wedgedness.

$$P_\mathrm{diff} \propto \frac{\pi e^{\frac{id^2}{2s}}}{2s} \times \left( \left( \mathrm{FC}\left[\frac{d}{\sqrt{2\pi}\sqrt{s}}\right] - \mathrm{FC}\left[\frac{d-2Ls}{\sqrt{2\pi}\sqrt{s}}\right] \right)^2 - \left( \mathrm{FS}\left[\frac{d}{\sqrt{2\pi}\sqrt{s}}\right] - \mathrm{FS}\left[\frac{d-2Ls}{\sqrt{2\pi}\sqrt{s}}\right] \right)^2 \right) \tag{47}$$

where FS and FC represent the Fresnel integrals. Fig. 12(a) shows the diffracted power as a function of the mologram diameter for a waveguide with a wedgedness of 5 nm/cm. There is no reason of fabricating a mologram larger than the size at which the diffracted power is at the maximum [blue]. However, this term is laborious to calculate and we therefore define another parameter to determine the phase mismatch. We define the dephasing length as the mologram size at which the first and the last molographic line will interfere completely destructively. Because we assume the change in waveguide thickness to be the main source of the effective refractive index gradient we substitute $\frac{dN}{dz} = \frac{dN}{dt_\mathrm{f}}\frac{dt_\mathrm{f}}{dz}$ into Eq. (45). The first and the last line will interfere destructively when the phase mismatch builds up to $\pi$. Solving

$$\frac{2\pi}{\lambda}\frac{dN}{dt_\mathrm{f}}\frac{dt_\mathrm{f}}{dz}\frac{D_\mathrm{deph}^2}{2} = \pi \tag{48}$$

yields an expression for the dephasing length.

$$D_\mathrm{deph} = \sqrt{\frac{\lambda}{\frac{dN}{dt_\mathrm{f}}\frac{dt_\mathrm{f}}{dz}}} \tag{49}$$

The dephasing length is indicated in green. From Fig. 12(a) it is apparent that the waveguides used for our experiments exhibited a wedgedness of less than 5 nm/cm because we did not observe any effect of the dephasing, which would have led to a deviation for larger molograms between the analytical model and the experiments in [see Fig. 5]. In Fig. 12(b) the maximum mologram size as a function of wedgedness is shown.

## V. ILLUMINATION SETUP AND FABRICATION OF MOLOGRAMS

We noted in our last publication that molograms with a better activation ratio could be fabricated by using a higher spatial and temporal coherence of the illumination source [5]. To achieve this, here a laser was used as light source. A different wavelength of 405 nm was chosen since these laser sources are cheap thanks to the blue ray disk. We used the same phase masks as in the last publication [optimized for 390 nm illumination] and nevertheless obtained molograms with nearly twice the surface mass modulation compared to the previous results [27 % vs 14 % of the ideally achievable modulation]. The optimal illumination dose lies between 2500-3000 mJ/cm$^2$ [compared to 284 mJ/cm$^2$ at 390 nm]. However, the achieved mass modulation is only weakly dependent on the illumination dose in the range 1800-3500 mJ/cm$^2$, resulting in a robust and reproducible illumination process. The illumination setup [2$^{\mathrm{nd}}$ generation] is displayed in Fig. 13. The mass density modulation for a dose of 2000 mJ/cm$^2$ determined by STED [stimulated emission depletion microscopy] and the molographic signal as a function of illumination dose are shown in Fig. 14 [same procedure as in [5]].

## VI. MOLOGRAPHIC MEASUREMENTS IN AIR

Molographic measurements in air, waveguide characterizations and speckle background analysis were carried out with the MoloReader in the configuration shown in Fig. 15. The entire setup is motorized such that all six measurement fields of a chip and all molograms on

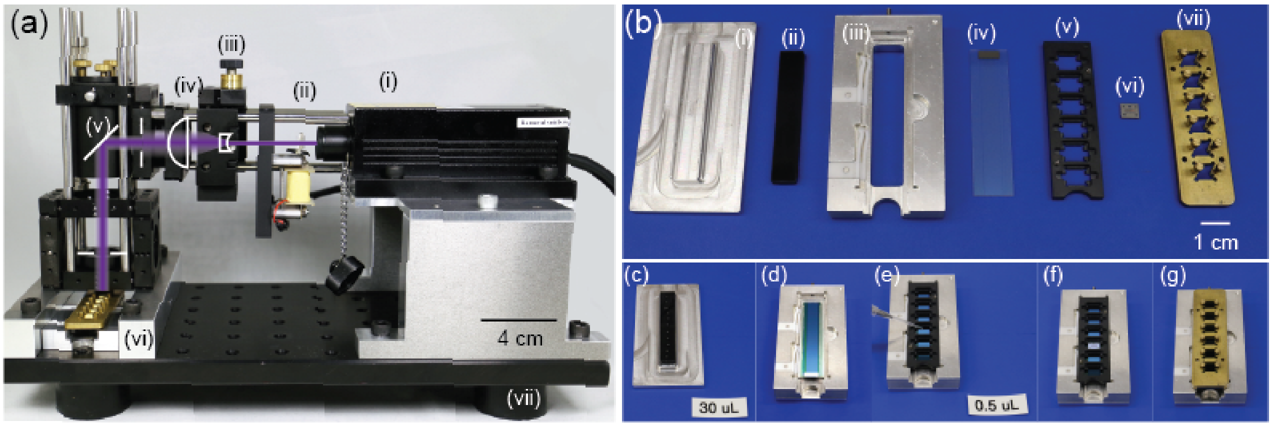


FIG. 13: Reactive immersion lithography setup (a) The second generation of the illumination setup for the creation of molograms. (i) A 405 nm solid state laser beam with a coherence length of a few 10 μm [Model RLTMLL-405-200-5 200 mW, Roithner Lasertechnik] is expanded by a factor 8.3 [Coherence lengths longer than this only create unwanted interferences with reflected beams] (ii) home-built solenoid shutter that controls the illumination time (iii) PCV f = -6mm lens [xy moveable, VIS 0 ° AR coated, #48265 Edmund optics], (iv) PCX lens [f = 50 mm, 405 nm V-Coat, #65465 Edmund optics], and deflected by an adjustable mirror [G063713000, Qioptiq] (v) to the chip and phase mask holder (vi). (vii) Sorbothane mounts [Edmund optics] for vibration isolation (b) Parts of the chip phase mask assembly holder (i) Aluminium support for black PDMS piece. (ii) carbon black [Cabot corporation] loaded [0.1 wt%] PDMS [Silgard 184, Dow Corning] piece in order to absorb transmitted radiation and avoid reflections. (iii) Aluminium holder with springs to secure molographic chip and mask holder. (iv) waveguide molographic chip. (v) machined PEEK mask holder for six phase masks. (vi) phase mask chip featuring thirty molographic structures. (vii) Brass mask to fix the chip with two additional brass pillars to avoid lateral movement during illumination. (c) - (g) Assembly of the chip and phase mask holder for lithography: (c) 30 μl of DMSO are applied to the PDMS piece to provide index matching between the chip back surface and the PDMS (d) waveguide chip inserted into the aluminium holder. (e) mask holder is inserted and 0.5 μl of the immersion medium [0.2% hydroxylamine in DMSO] is pipetted onto the molographic field. (f) one of the six phase mask inserted into the holder. (g) The final chip phase mask assembly as it is used in the illumination setup.

each of them can be separately measured. The arrangement of motors, microscope and the fiber coupled laser are displayed in Fig. 15(a). The arrangement can be separated in a moveable microscopy assembly [x,z] and a moveable chip assembly [y]. Each of the stepper motors had a small manual microstage [UMR3.5, Newport] on the other assembly for fine adjustments [microscope to beam alignment and coupling grating to center of rotation alignment]. A MetalVelvet$^{\mathrm{TM}}$ Adhesive [ACM coatings] coated aluminium cover with openings for the coupling beam was used to block the direct stray light [Fig. 15(b)]. This stray light mainly originated from the adjustable aperture whose function was to control the beam diameter. Fig. 15(c) shows a propagating TE mode and the small MetalVelvet$^{\mathrm{TM}}$ Adhesive pieces that were used to protect the microscope from excessive stray light as well as the photodiode for measuring the out-coupled power.

### A. Effective focal point distance and adjusted depth of field

The distance measured between the chip surface and the focal point differ from the focal distance that is expected by the design of the mologram [900 μm]. This is a consequence of the refraction of light due to the optical interface. As evident from Fig. 16, two aspects contribute to the difference between the measured and the designed focal length: First, the distance seen by the objective appears to be shorter than the real distance due to the transmission into a denser medium [Fig. 16(a)]. By knowledge of the real distance [chip thickness: 700 μm], the apparent chip thickness can be calculated as

$$d_{\mathrm{a}} = \frac{n_{\mathrm{s}}}{n_{\mathrm{o}}} d_{\mathrm{r}} \tag{50}$$

which amounts to a value of 460 μm. Second, the scattered rays are refracted at the bottom interface of the chip. The remaining 200 μm from the bottom surface will be compressed by the refractive index of the glass substrate by $1/n_{\mathrm{s}}$ yielding a focal distance of 831 μm with respect to the chip surface [see Fig. 16(b) and (c)],

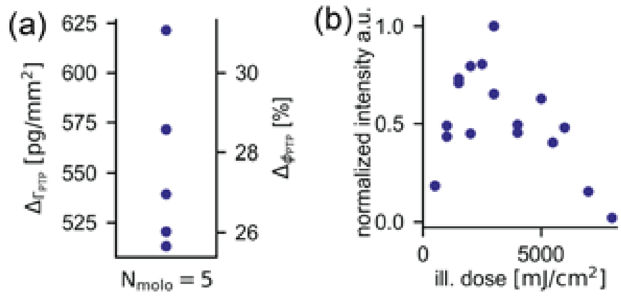


FIG. 14: Characterization of the illumination setup (a) Activation and surface mass density modulation from STED [Stimulated Emission Depletion microscopy] images. The exposure dose was 2000 mJ/cm$^2$ and five different molograms were investigated in the same way as described in Supplementary Fig. 6 of our previous work [5]. The median of the activation modulation $\Delta_{\phi_{\mathrm{PTP}}}$ amounted to 27 % with a 95 % confidence in the interval [25.6, 31] %. The median of the Peak-to-Peak surface mass density modulation $\Delta_{\Gamma_{\mathrm{PTP}}}$ amounted to 540 pg/mm$^2$ when incubated with 1 µM of SAv [2000 pg/mm$^2$ surface coverage for 100 % activation] with a confidence of 95 % to be in the interval [513, 621] pg/mm$^2$. (b) The measured mologram intensity as a function of illumination dose at 405 nm for SAv molograms. The illumination dose of 2000 mJ/cm$^2$ used in this manuscript is close to the maximum of the curve and has the advantage that the ridges are not yet fully saturated.

such that the apparent focal distance is approximately at 592 µm. Evidently, this exactly corresponds to the focal length of this mologram on the air side as requested in order to exhibit the same numerical aperture on both sides by Snell's law.

### B. Shape of the Airy disk with and without central bragg recess area

Fig. 17 shows that the distortion of the Airy disk compared to a diffraction-limited lens is mainly caused by the central Bragg area which breaks the radial symmetry.

### C. Power calculations for the molograms in Fig. 5

The power in the waveguide was calculated from the in-coupled beam diameter [1 mm set by an adjustable aperture Fig. 15] and the out-coupled power measured by a photodiode. The distance of the mologram out-coupling grating was different for each mologram [spacing 400 µm, average distance to out-coupling grating was 6 mm] and the power in the waveguide at the location of the mologram was calculated by the determined damping constant of this waveguide [6.5 dB/cm] by the MoloReader.

## VII. MODELS FOR BACKGROUND SCATTERING

### A. Approximative formula for the background intensity in the focal spot

The exact equation to calculate the intensity due to a distributed scattering mechanism giving rise to an isotropic scattering leakage $\alpha_{\mathrm{sca}}$ is

$$I_{\mathrm{bg}} = \alpha_{\mathrm{sca}} P_{\mathrm{wg}} \int_0^{2\pi} \int_0^{D/2} \frac{e^{-\alpha(\rho \cos\phi)}}{4\pi(f^2+\rho^2)} \rho d\rho d\phi \tag{51}$$

However, there is no analytical solution for this expression. To simplify the calculations we consider the entire background power as a spherical wave originating from the middle of the mologram, which is then collected by an objective of a given numerical aperture. We essentially neglect free space attenuation. However, this effect is small and we also neglect free space attenuation of the signal. Signal and background are affected in the same way by free space attenuation. To obtain an analytical expression, we approximate the total radiated background power [in Watts] by

$$P_{\mathrm{rad}} = D P_{\mathrm{wg}} \left(1 - \exp\left(-\alpha_{\mathrm{sca}} \frac{D\pi}{4}\right)\right) \approx \frac{D^2 \alpha_{\mathrm{sca}} \pi}{4} P_{\mathrm{wg}} \tag{52}$$

Since we assume that this power is distributed over a solid angle of $4\pi$ the intensity in the focal spot can be expressed in terms of the numerical aperture of the objective.

$$I_{\mathrm{bg}} = \frac{P_{\mathrm{rad}} n_{\mathrm{s}}^2}{4\pi f^2} = \frac{D^2 n_{\mathrm{s}}^2 \alpha_{\mathrm{sca}}}{16 f^2} P_{\mathrm{wg}} = \frac{1}{4} \mathrm{NA}^2 \alpha_{\mathrm{sca}} P_{\mathrm{wg}} \tag{53}$$

This equation underestimates the total intensity in the focal spot. Surprisingly, the error does not depend on the leakage parameter. It only depends on the numerical aperture, with larger errors for larger numerical apertures as expected. The error for a 0.1 NA objective is below 1 % and rises to roughly 25 % for 0.6 NA objectives. Yet, as described in the main manuscript the scattering is not isotropic. Therefore, Eq. (52) is corrected by the anisotropy parameter $a_{\mathrm{ani}}$.

### B. Sidewall roughness scattering

In this section we derive expressions for the attenuation constant and the scattering leakage. They can be computed from the statistical properties of the interfaces - namely the correlation length $L_{\mathrm{c}}$ and the RMS-roughness $\sigma$. The derivation was adopted from [21] and [22]. It was generalized to cover the case of an asymmetric slab waveguide. In these papers, the difference in

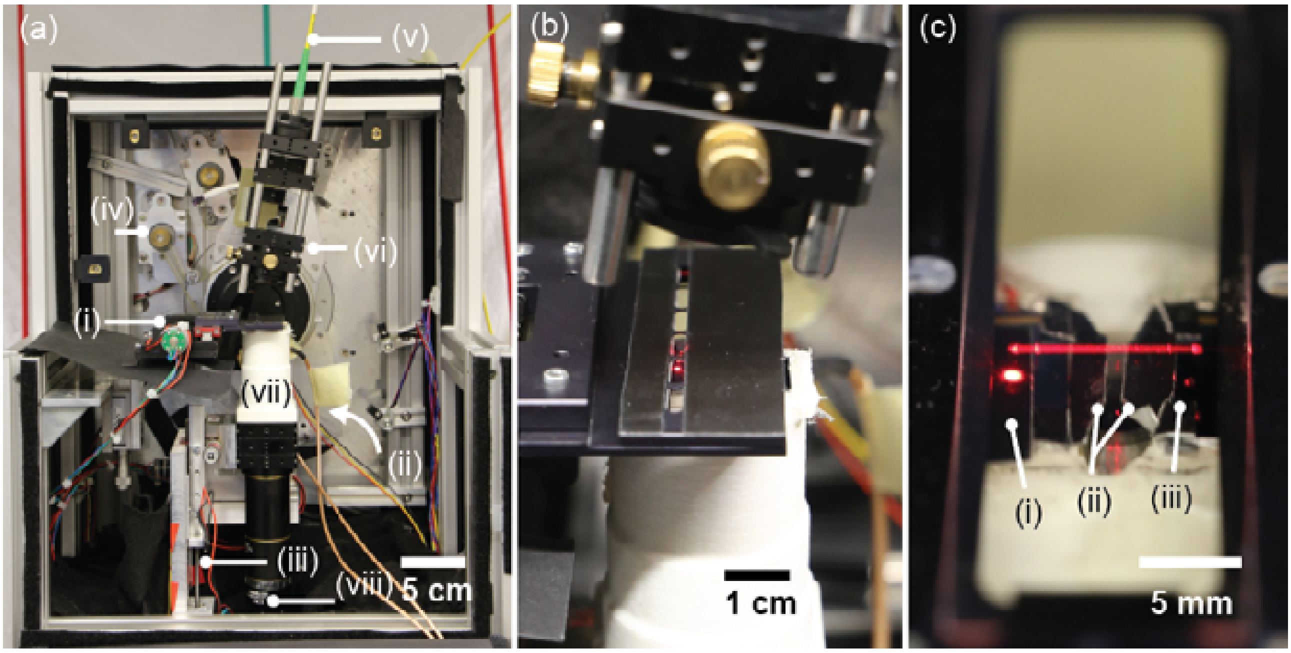


FIG. 15: MoloReader configuration for measurements in air (a) Stepper motor for movement of chip y-axis (i), movement of microscope x (ii) and z-axis (iii) and for adjusting the in-coupling angle (iv). Motors (i) - (iii) were obtained from Faulhaber Inc, Models (i) - (ii) AM1524 [M3x0.5 thread and M2x0.2 thread] and AM2224 [M3x0.5 thread] for (iii) controlled by MCST 3601 motor controllers, Motor (iv) is an ancient RDM545 model [Berger Lahr] controlled by a Raspberry Pi 2 Model B and a D225 5 phase stepper motor control card. (v) APC fiber-coupled HeNe Laser [HNL020L-EC 2mW, Thorlabs]. (vi) Moveable adjustable aperture [set to 1mm for most of the experiments] (vii) Imaging system consisting of a standard DIN 20x 0.4 NA achromatic objective [Edmund Optics] (vii) and a C-Mount tube with CMOS Camera (viii) [IDS Imaging Development Systems GmbH, Model UI-3480CP Rev.2, 2.2 µm pixelsize, 2560 x 1920 pixels]. (b) chip holder with straylight cover. This setup configuration was used to acquire all the experimental data except the noise level measurements in Fig. 9 and movies. (c) Zeptochip with propagating TE mode. (i) Standard MetalVelvet$^{\mathrm{TM}}$ Adhesive [ACM coatings] to absorb most of the in-coupled light beneath the chip. (ii) additional light absorbing adhesive to protect the microscopy objective against stray light from the in-coupling and out-coupling grating. (iii) Anode grounded photodiode to measure the out-coupled light [FDS1010, Thorlabs] via a bias module [PBM42, Thorlabs] and a DAQ system [U6, Labjack]. Load resistance was adapted to the light levels [1 kΩ].

notation compared to this publication is worth noticing. The thickness of the waveguide film $t_\mathrm{f}$ is defined as $2d$ and the coordinate system is defined in a different manner [to transform from our coordinate system to theirs: $x \to z$, $y \to x$, $z \to y$]. The refractive index distribution of an asymmetric waveguide can be written in the following way

$$\begin{aligned} n^2 &= n_c^2 + \left(n_\mathrm{f}^2 - n_\mathrm{c}^2\right) U\left[f(x) - z\right] \\ &\quad - \left(n_\mathrm{f}^2 - n_\mathrm{s}^2\right) U\left[-\left(t_\mathrm{f} + f(x) + z\right)\right] \end{aligned} \tag{54}$$

where $U$ is the unit step function and $f(z)$ is the function of the sidewall roughness: $U[a] = 0$ if $a < 0$ and $U[a] = 1$ if $a > 0$. Following the procedure in Ref. [21] this leads to a slightly different solution for the perturbed fields of the asymmetric waveguide [symmetric case Eq. (7) in Ref. [21]].

$$\begin{aligned} E_y(x,z) = & \int_{-\infty}^{\infty}\int_{-\infty}^{\infty} k_0^2 \left(n_\mathrm{f}^2 - n_\mathrm{c}^2\right) U\left[f(x') - z'\right] \\ & \times E_{y0}(x,z) G(x,x',z,z') dy dz' \\ & - \int_{-\infty}^{\infty}\int_{-\infty}^{\infty} k_0^2 \left(n_\mathrm{f}^2 - n_\mathrm{s}^2\right) U\left[-\left(t_\mathrm{f} + f(x') + z'\right)\right] \\ & \times E_{y0}(x,z) G(x,x',z,z') dy dz' \end{aligned} \tag{55}$$

where $G$ is the Green's function of the waveguide. As in Ref. [21] we will assume the two sidewalls to be non-correlated. Thus, we can treat them separately and add their contribution as done in Ref. [21]. Therefore, we can solve the integral over $dz'$ [see Eq. (9) in Ref. [21]] using a first order Taylor approximation resulting in

$$\begin{aligned} E_y(x,z) &= \frac{\sqrt{2}}{2} k_0^2 \left(\phi(0)\left(n_\mathrm{f}^2 - n_\mathrm{c}^2\right) + \phi(-t_\mathrm{f})\left(n_\mathrm{f}^2 - n_s^2\right)\right) \\ &\quad \times \int_{-\infty}^{\infty} e^{-i\beta x'} G(x,x',z,z') dx' \end{aligned} \tag{56}$$

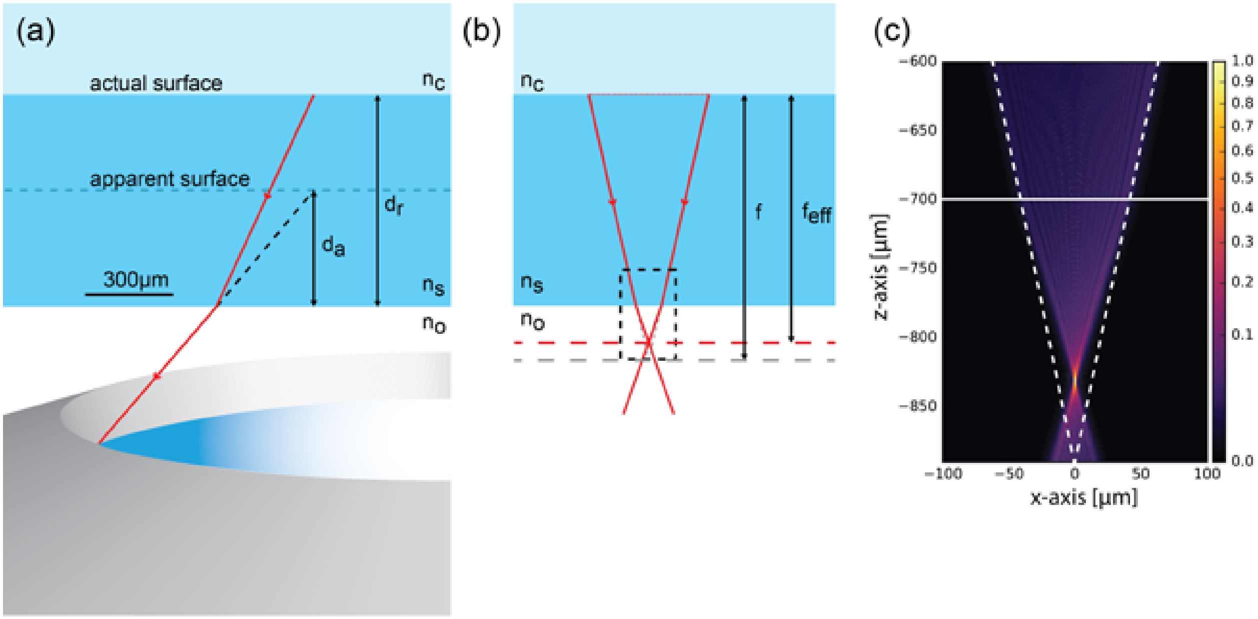


FIG. 16: Difference of the measured focal plane and the designed focal plane. (a) The optical interface induces a difference between the real and the apparent chip surface. The mologram is designed for a focal distance of 900 μm in a medium of $n_s = 1.521$. (b) Since the chip thickness is only 700 μm, the rays are refracted due to the refractive index change of the media [$n_s = 1.521$, $n_0 = 1$]. (c) An upward shift of the focal point is clearly observable if the change of refractive index is introduced in the simulations. The distance measured between the chip surface and the focal point $f_{\text{eff}}$ was approximately 592 μm which coincides with the calculations.

where $\phi$ is the normalized electric field of the unperturbed waveguide.

$$\phi^2(z) = \frac{|E_y(z)|^2}{\int\limits_{-\infty}^{\infty} |E_y(z)|^2 dz} \tag{57}$$

For the integration over $dx'$ we make use of the Fourier Transform of the Green's function. Thus, Eq. (56) is Fourier transformed to the wavenumber domain [$k_x$, $k_z$]. Then the equation is transferred back into the spacial [$x$, $z$] domain by the inverse Fourier Transform. For the inverse Fourier Transformation we need to consider that in contrast to the symmetric waveguide covered by Ref. [21] scattering into the upper half-space is not identical to scattering into the lower half-space. Thus, the integral over $dk_z$ [$dk_y$ in Ref. [21] Eq. (11)] needs to be split into two separate integrals. One covers scattering into the upper half-space and the other one covers the scattering into the lower half-space. However, because we are not interested in the phase information and due to the even character of the real part the result does not complicate much.

$$\text{Re}\left\{\int\limits_{0}^{\infty} \frac{e^{ik_z z}}{n_c^2 k_0^2 - k_y^2 - k_z^2} dk_z + \int\limits_{-\infty}^{0} \frac{e^{ik_z z}}{n_s^2 k_0^2 - k_y^2 - k_z^2} dk_z\right\} = \frac{1}{2}\text{Re}\left\{\int\limits_{-\infty}^{\infty} \frac{e^{ik_z z}}{n_c^2 k_0^2 - k_y^2 - k_z^2} dk_z + \int\limits_{-\infty}^{\infty} \frac{e^{ik_z z}}{n_s^2 k_0^2 - k_y^2 - k_z^2} dk_z\right\} \tag{58}$$

We end up with four different contributions to the attenuation constant, one for each combination of sidewall and upper respectively lower half-space scattering. We can apply all further steps in Ref. [21] to each of the four contributions and therefore directly write our result in the form of Eq. (16) in Ref. [21]. The factorization of the four contributions reads as

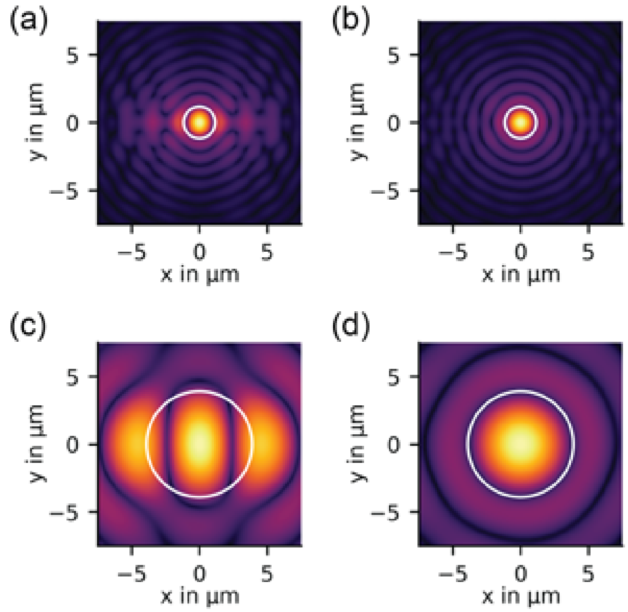


FIG. 17: Shape of the Airy disk for two molograms [0.33 and 0.1 NA] with (a), (c) and without central (b), (d) Bragg recess area. The white circle is the size of Airy disk of the diffraction-limited lens with the same NA.

$$\begin{aligned}\alpha_{\mathrm{sca,r}} &= \frac{1}{4}\frac{k_0^3}{4\pi n_{\mathrm{f}}} \\ &\times\left(\phi^2\left(0\right)\left(n_{\mathrm{f}}^2-n_{\mathrm{c}}^2\right)^2+\phi^2\left(-t_{\mathrm{f}}\right)\left(n_{\mathrm{f}}^2-n_{\mathrm{c}}^2\right)^2\right) \\ &\times\left(\int_0^{\pi}\int_{-\infty}^{\infty}R(u)e^{i(\beta-n_{\mathrm{c}}k_0\cos\theta)u}du d\theta\right. \\ &\left.+\int_0^{\pi}\int_{-\infty}^{\infty}R(u)e^{i(\beta-n_{\mathrm{s}}k_0\cos\theta)u}du d\theta\right) \end{aligned} \tag{59}$$

where the first bracket contains the two sidewall contributions and the second one contains the upper and lower half-space scattering. $R\left(u\right)$ is the correlation function of the surface roughness. The angle $\theta$ is defined such that it is zero in the forward scattering direction. Next, we use the expressions [Eqs. (1.3-16), (1.3-17) and (1.3-46, 47)] given in Ref. [6] for the electric field of the fundamental TE mode of the asymmetric waveguide to get an expression for the normalized fields at the two interfaces $\phi^2\left(0\right)$ and $\phi^2\left(-t_{\mathrm{f}}\right)$

$$\phi^2(0)=\frac{A^2}{\left|E_{\mathrm{tot}}\right|^2}=\frac{A^2N}{2\mu_0c_0P}=\frac{4\kappa^2\omega N}{2\left|\beta\right|t_{\mathrm{eff}}\left(\kappa^2+\delta^2\right)c_0} \tag{60a}$$

$$\begin{aligned}\phi^2(-t_{\mathrm{f}}) &= \frac{\left(A\cos(\kappa t_{\mathrm{f}})-B\sin(\kappa t_{\mathrm{f}})\right)^2}{\left|E_{\mathrm{tot}}\right|^2} \\ &= \left(\cos(\kappa t_{\mathrm{f}})+\frac{\delta}{\kappa}\sin(\kappa t_{\mathrm{f}})\right)^2 \\ &\times\frac{4\kappa^2\omega N}{2\left|\beta\right|\left(d+\frac{1}{\gamma}+\frac{1}{\delta}\right)\left(\kappa^2+\delta^2\right)c_0}\end{aligned} \tag{60b}$$

where the relation of the power and the total field is just the integrated Poynting flux in $z$ and $\gamma$, $\kappa$ and $\delta$ are the $z$ components of the wave vector $k$ in the three media: substrate, film and cover [6]. They can be expressed in function of their corresponding refractive index and of the effective refractive index $N$.

$$\gamma^2=\beta^2\frac{N^2-n_{\mathrm{s}}^2}{N^2} \tag{61a}$$

$$\kappa^2=\beta^2\frac{n_{\mathrm{f}}^2-N^2}{N^2} \tag{61b}$$

$$\delta^2=\beta^2\frac{N^2-n_{\mathrm{c}}^2}{N^2} \tag{61c}$$

Furthermore, it is convenient to state the following relation,

$$\frac{\kappa^2}{\kappa^2+\delta^2}=\frac{n_{\mathrm{f}}^2-N^2}{n_{\mathrm{f}}^2-n_{\mathrm{c}}^2} \tag{62}$$

which allows the normalized fields at the two interfaces to be written in a more concise way.

$$\phi^2(0)=\frac{2\left(n_{\mathrm{f}}^2-N^2\right)}{t_{\mathrm{eff}}\left(n_{\mathrm{f}}^2-n_{\mathrm{c}}^2\right)} \tag{63a}$$

$$\begin{aligned}\phi^2(-t_{\mathrm{f}}) &= \frac{2\left(n_{\mathrm{f}}^2-N^2\right)}{t_{\mathrm{eff}}\left(n_{\mathrm{f}}^2-n_{\mathrm{c}}^2\right)} \\ &\times\left(\cos\left(t_{\mathrm{f}}\beta\frac{\left(n_{\mathrm{f}}^2-N^2\right)^{1/2}}{N}\right)\right. \\ &\left.+\frac{\left(N^2-n_{\mathrm{c}}^2\right)^{1/2}}{\left(n_{\mathrm{f}}^2-N^2\right)^{1/2}}\sin\left(t_{\mathrm{f}}\beta\frac{\left(n_{\mathrm{f}}^2-N^2\right)^{1/2}}{N}\right)\right)^2\end{aligned} \tag{63b}$$

By substituting these values into Eq. (59) we get for the damping constant due to surface roughness

$$\alpha_{\mathrm{sca,r}} = \frac{1}{2}\frac{\left(n_{\mathrm{f}}^2-N^2\right)}{t_{\mathrm{eff}}\left(n_{\mathrm{f}}^2-n_{\mathrm{c}}^2\right)}\frac{k_0^3}{4\pi n_{\mathrm{f}}} \times\left(\left(n_{\mathrm{f}}^2-n_{\mathrm{c}}^2\right)^2+J^2\left(n_{\mathrm{f}}^2-n_{\mathrm{s}}^2\right)^2\right) \times\left(\int_0^{\pi}\int_{-\infty}^{\infty}R(u)e^{i(\beta-n_{\mathrm{c}}k_0\cos\theta)u}dud\theta + \int_0^{\pi}\int_{-\infty}^{\infty}R(u)e^{i(\beta-n_{\mathrm{s}}k_0\cos\theta)u}dud\theta\right) \quad (64)$$

where we define $J$ as the asymmetry parameter of the waveguide.

$$J = \cos\left(t_{\mathrm{f}}\beta\frac{\left(n_{\mathrm{f}}^2-N^2\right)^{1/2}}{N}\right) + \frac{\left(N^2-n_{\mathrm{c}}^2\right)^{1/2}}{\left(n_{\mathrm{f}}^2-N^2\right)^{1/2}}\sin\left(t_{\mathrm{f}}\beta\frac{\left(n_{\mathrm{f}}^2-N^2\right)^{1/2}}{N}\right) \quad (65)$$

It is important to note that attenuation due to scattering into waveguide modes is not accounted for by this equation. The integral is solved in Ref. [22] with the assumption of an exponential form of the roughness correlation function $R(u)=\sigma^2\exp\left(-\frac{|u|}{L_{\mathrm{c}}}\right)$. This can be used to determine the attenuation coefficient of the sidewall scattering $\alpha_{\mathrm{sca,r}}$. For completeness, this is done at the end of this section. However, in order to determine the background intensity we are interested in finding an expression for the scattering leakage $a_{\mathrm{ani,r}}\alpha_{\mathrm{sca,r}}$. The anisotropic scattering is illustrated in Fig. 6 in the manuscript.

Since we are interested only in the radiation into the substrate region, only the second integral needs to be considered in Eq. (64). The boundaries of the integral over the angle $\theta$ need to be adapted, since only scattered rays captured by the numerical aperture matter. The scattering leakage contribution that radiates into the numerical aperture of the objective reads

$$\alpha_{\mathrm{NA,real}} = \frac{1}{2}\frac{\left(n_{\mathrm{f}}^2-N^2\right)}{t_{\mathrm{eff}}\left(n_{\mathrm{f}}^2-n_{\mathrm{c}}^2\right)}\frac{k_0^3}{4\pi n_{\mathrm{f}}} \times\left(\left(n_{\mathrm{f}}^2-n_{\mathrm{c}}^2\right)^2+J^2\left(n_{\mathrm{f}}^2-n_{\mathrm{s}}^2\right)^2\right) \times\int_{\frac{\pi}{2}-\frac{\mathrm{NA}}{n_{\mathrm{s}}}}^{\frac{\pi}{2}+\frac{\mathrm{NA}}{n_{\mathrm{s}}}}\int_{-\infty}^{\infty}R(u)e^{i(\beta-n_{\mathrm{s}}k_0\cos\theta)u}dud\theta \quad (66)$$

We have approximated the integral boundaries by $\arcsin\left(\frac{\pi}{2}\pm\frac{\mathrm{NA}}{n_{\mathrm{s}}}\right)\approx\pm\frac{\mathrm{NA}}{n_{\mathrm{s}}}$. The anisotropy parameter is then simply this quantity divided by the damping constant weighted by the angular contribution of the numerical aperture [This weighting factor is $\frac{1}{2\pi}\frac{2\cdot\mathrm{NA}}{n_{\mathrm{s}}}$ since the damping constant $\alpha_{\mathrm{sca,r}}$ is obtained by integration over $2\pi$ in Eq. (64)]. In this normalization, we did not account for the different relative contribution of the angles within the numerical aperture [The center of the mologram with $\theta=\frac{\pi}{2}$ gives a larger contribution than the edges.].

$$a_{\mathrm{ani}} = \frac{\alpha_{\mathrm{NA,real}}}{\alpha_{\mathrm{NA,iso}}} = \frac{\alpha_{\mathrm{NA,real}}}{\alpha_{\mathrm{sca,r}}\frac{1}{2\pi}\frac{2\cdot\mathrm{NA}}{n_{\mathrm{s}}}} \quad (67)$$

As in Ref. [22] we assume an exponential form of the autocorrelation function. Thus, evaluating the integral as described in Ref. [22]

$$\int_{\frac{\pi}{2}-\frac{\mathrm{NA}}{n_{\mathrm{s}}}}^{\frac{\pi}{2}+\frac{\mathrm{NA}}{n_{\mathrm{s}}}}\int_{-\infty}^{\infty}R(u)e^{i(\beta-n_{\mathrm{s}}k_0\cos\theta)u}dud\theta = 2\sigma^2L_c\int_{\frac{\pi}{2}-\frac{\mathrm{NA}}{n_{\mathrm{s}}}}^{\frac{\pi}{2}+\frac{\mathrm{NA}}{n_{\mathrm{s}}}}\frac{1}{1+\left(\left(\beta-kn_{\mathrm{s}}\cos\theta\right)L_{\mathrm{c}}\right)^2}d\theta \quad (68)$$

The scattering leakage then reads

$$a_{\mathrm{ani,r}}\alpha_{\mathrm{sca,r}} = \frac{\pi n_{\mathrm{s}}}{\mathrm{NA}}\frac{1}{2}\frac{\left(n_{\mathrm{f}}^2-N^2\right)}{t_{\mathrm{eff}}\left(n_{\mathrm{f}}^2-n_{\mathrm{c}}^2\right)}\frac{k_0^3}{4\pi n_{\mathrm{f}}} \times\left(\left(n_{\mathrm{f}}^2-n_{\mathrm{c}}^2\right)^2+J^2\left(n_{\mathrm{f}}^2-n_{\mathrm{s}}^2\right)^2\right) \times 2\sigma^2L_c\int_{\frac{\pi}{2}-\frac{\mathrm{NA}}{n_{\mathrm{s}}}}^{\frac{\pi}{2}+\frac{\mathrm{NA}}{n_{\mathrm{s}}}}\frac{1}{1+\left(\left(\beta-kn_{\mathrm{s}}\cos\theta\right)L_{\mathrm{c}}\right)^2}d\theta \quad (69)$$

This expression can be rewritten such that

$$a_{\mathrm{ani,r}}\alpha_{\mathrm{sca,r}} = \frac{\pi n_{\mathrm{s}}}{\mathrm{NA}}\frac{\pi\left(n_{\mathrm{f}}^2-N^2\right)}{t_{\mathrm{eff}}\left(n_{\mathrm{f}}^2-n_{\mathrm{c}}^2\right)}\frac{\sigma^2}{\lambda^2Nn_{\mathrm{f}}} \times\left(\left(n_{\mathrm{f}}^2-n_{\mathrm{c}}^2\right)^2+J^2\left(n_{\mathrm{f}}^2-n_{\mathrm{s}}^2\right)^2\right) \times L_c\beta\int_{\frac{\pi}{2}-\frac{\mathrm{NA}}{n_{\mathrm{s}}}}^{\frac{\pi}{2}+\frac{\mathrm{NA}}{n_{\mathrm{s}}}}\frac{1}{1+\left(\left(\beta-kn_{\mathrm{s}}\cos\theta\right)L_{\mathrm{c}}\right)^2}d\theta \quad (70)$$

The integral could be solved analytically. However, it yields an elaborate expression from which no practical information is gained. The integration is not performed here and the integral was evaluated numerically.

For the sake of completeness, we also derive the attenuation coefficient for the sidewall roughness scattering as mentioned above. As described in Ref. [22] the integrals in Eq. (64) can be solved analytically.

$$\int_0^{\pi}\int_{-\infty}^{\infty} R(u)e^{i(\beta-n_ik_0\cos\theta)u}dud\theta = 2\sigma^2 L_c\int_0^{\pi}\frac{1}{1+\left(\left(\beta-kn_i\cos\theta\right)L_\mathrm{c}\right)^2}d\theta = \sqrt{2}\pi\sigma^2 L_c\frac{\left(\left(4\beta^2L_\mathrm{c}^2+\left(1-L_\mathrm{c}^2\left(\beta^2-n_i^2k_0^2\right)\right)^2\right)^{1/2}+1-L_\mathrm{c}^2\left(\beta^2-n_i^2k_0^2\right)\right)^{1/2}}{\left(4\beta^2L_\mathrm{c}^2+\left(1-L_\mathrm{c}^2\left(\beta^2-n_i^2k_0^2\right)\right)^2\right)^{1/2}} \tag{71}$$

where $i$ stands for the substrate s or the cover c respectively. In order to get a dimensionless term we expand with $\beta/\beta$ and get,

$$\int_0^{\pi}\int_{-\infty}^{\infty} R(u)e^{i(\beta-n_ik_0\cos\theta)u}dud\theta = \frac{\sqrt{2}\pi\sigma^2}{\beta}F_i\left(L_\mathrm{c},\beta\right) \tag{72}$$

where $F_i$ is dimensionless and expressed as

$$F_i\left(L_\mathrm{c},\beta\right) = L_\mathrm{c}\beta\frac{\left(\left(4\beta^2L_\mathrm{c}^2+\left(1-L_\mathrm{c}^2\left(\beta^2-n_i^2k_0^2\right)\right)^2\right)^{1/2}+1-L_\mathrm{c}^2\left(\beta^2-n_i^2k_0^2\right)\right)^{1/2}}{\left(4\beta^2L_\mathrm{c}^2+\left(1-L_\mathrm{c}^2\left(\beta^2-n_i^2k_0^2\right)\right)^2\right)^{1/2}} \tag{73}$$

Thus, the attenuation constant yields

$$\alpha_{\mathrm{sca,r}} = \frac{\left(n_\mathrm{f}^2-N^2\right)}{t_\mathrm{eff}\left(n_\mathrm{f}^2-n_\mathrm{c}^2\right)}\frac{k_0^3}{4\pi n_\mathrm{f}}\frac{1}{2}\frac{\sqrt{2}\pi\sigma^2}{\beta} \times\left(\left(n_\mathrm{f}^2-n_\mathrm{c}^2\right)^2+J^2\left(n_\mathrm{f}^2-n_\mathrm{s}^2\right)^2\right) \times\left(F_\mathrm{c}\left(L_\mathrm{c},\beta\right)+F_\mathrm{s}\left(L_\mathrm{c},\beta\right)\right) \tag{74}$$

which can be written as

$$\alpha_{\mathrm{sca,r}} = \frac{\sqrt{2}}{2}\pi^2\frac{\sigma^2}{\lambda^2}\frac{\left(n_\mathrm{f}^2-N^2\right)}{Nt_\mathrm{eff}\left(n_\mathrm{f}^2-n_\mathrm{c}^2\right)n_\mathrm{f}} \times\left(\left(n_\mathrm{f}^2-n_\mathrm{c}^2\right)^2+J^2\left(n_\mathrm{f}^2-n_\mathrm{s}^2\right)^2\right) \times\left(F_\mathrm{c}\left(L_\mathrm{c},\beta\right)+F_\mathrm{s}\left(L_\mathrm{c},\beta\right)\right) \tag{75}$$

## VIII. WAVEGUIDE AND BACKGROUND CHARACTERIZATION

In this section, we first show the validation of the model for the scattering leakage due to waveguide surface scattering and the necessary characterization to assess the suitability of a waveguide for molography. The goal is to determine the total scattering leakage and in addition whether it is dominated by surface or volume scattering.

### A. Validation of the model for scattering leakage due to waveguide surface scattering

To validate the model for the scattering leakage the statistical properties of the surface $L_c$ and $\sigma$ must be acquired by a suitable technique - i.e. AFM. The AFM measurement resulted in an RMS roughness of 0.6 nm. It is not trivial to determine the correlation length from the AFM measurement since there are several exponen-

tial decays superimposed on each other. This results in a large uncertainty for the model of the surface scattering leakage [Eq. (70)]. The AFM data suggest a range between 100 nm and 900 nm for the correlation length, and the best fit yields a correlation length of 588 nm. Using Eq. (70) this leads to a scattering leakage of 6.65 /m, whereas 3.12 /m have been measured experimentally [Figs. 18 and 19]. A corresponding background intensity of 5.3 mW/m$^2$ for a $P_{\mathrm{wg}}$ of 0.02 W/m and an NA of 0.4 was calculated with the help of Eq. (5). Experimentally, 2.7 mW/m$^2$ was measured for an average waveguide [see next sections]. When addressing $\alpha_{\mathrm{sca,r}}$ and $a_{\mathrm{ani,r}}$ separately, the model predicts for $\alpha_{\mathrm{sca,r}}$ 36.2 /m [1.57 dB/cm] whereas 57.8 /m [2.51 dB/cm] have been measured [Fig. 18]. For $a_{\mathrm{ani,r}}$ the model yields 0.22 compared to 0.054 being measured experimentally [Fig. 19]. This divergence of absolute values between model and measurements are due to the following issues of the model: the uncertainty in the correlation length, neglecting guided to guided mode scattering, the model being two-dimensional and the assumption of uncorrelated sidewalls. In addition, some inaccuracies can arise from the limited precision of the measurement of the power carried by the waveguide mode. Nevertheless, the model can be used to provide a first estimate for the scattering leakage from an AFM measurement.

### B. Relative importance of surface to volume scattering

The relative importance of volume to surface scattering can be investigated by measuring the ratio of the scattered intensity with two different cover media, since volume scattering will be hardly affected by the change in cover medium. Furthermore, the model for the surface roughness can be used to estimate the reduction of intensity from the surface scattering. We chose air and index matching oil [Immersol 518F, Zeiss] as the cover media. For the difference in scattered field intensity between oil and air, the model for the surface roughness predicts a reduction of a factor of 1.6 of the scattered intensity due to the lower index contrast at the cover interface. Experimentally, the intensity dropped by a factor 2.3. The higher experimental value can be explained by the change from an asymmetric to a symmetric waveguide upon oil immersion [roughly a reduction in factor 1.5 for a dipole]. A stronger scattering into the optical denser half-space in the asymmetric case is not considered in the model since the signal is affected in the same way [15]. Therefore, the reduction of a factor 2.3 is a strong indication that surface scattering is the dominant background source because volume scattering is hardly affected by the change in cover medium. If volume scattering were dominant, one would expect a much lower reduction of the background intensity only caused by the symmetry change of the waveguide [roughly 1.5].

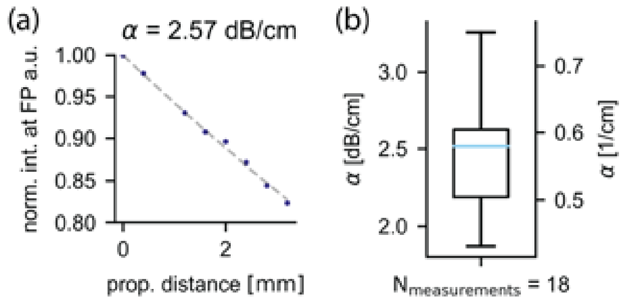


FIG. 18: Waveguide damping constant characterization. (a) typical exponential decay of the scattered light of a waveguide mode (b) Spread of the acquired damping constants. The median was 2.51 dB/cm or 0.58 1/cm.

### C. Damping constant characterization

The damping constants of coating stripped [30 s $O_2$ Plasma, 10 min US in DI water] ZeptoMark chips were measured on the MoloReader. Prior to measurement, stage movement and mode propagation direction were aligned. Stray light images were acquired 100 μm below the chip surface and the mean of each image was used for exponential fitting. Per damping trace six images spaced by 400 μm were acquired. The damping constants were measured on three chips at six different locations each. The median damping constant amounted to 2.51 dB/cm [Fig. 18]. Other attenuation constants stated in the manuscript were measured by this method for the corresponding chips.

### D. Experimental determination of scattering leakage and anisotropy of scattering

The scattering leakage can be determined by simultaneously measuring the power in the waveguide by the MoloReader and the intensity at a sufficient distance and using Eq. (5). We performed this characterization for the $Ta_2O_5$ waveguide in air. The anisotropy coefficient can be determined by dividing the scattering leakage with the attenuation constant. Fig. 19(a) shows the measured intensity normalized to a power of 0.02 W/m in the waveguide compared to what was expected if the scattered power would be distributed uniformly over the solid angle. Fig. 19(b) shows the box plot of the anisotropic scattering coefficient from 180 measurements and Fig. 19(c) the non-normalized intensity values plotted against the corresponding power in the waveguide.

### E. AFM characterization of surface roughness

AFM was used to determine the surface roughness [Fig. 20(a)]. The chip was mounted on the micrometer positioning stage of a Dimension Icon AFM [Bruker, Santa

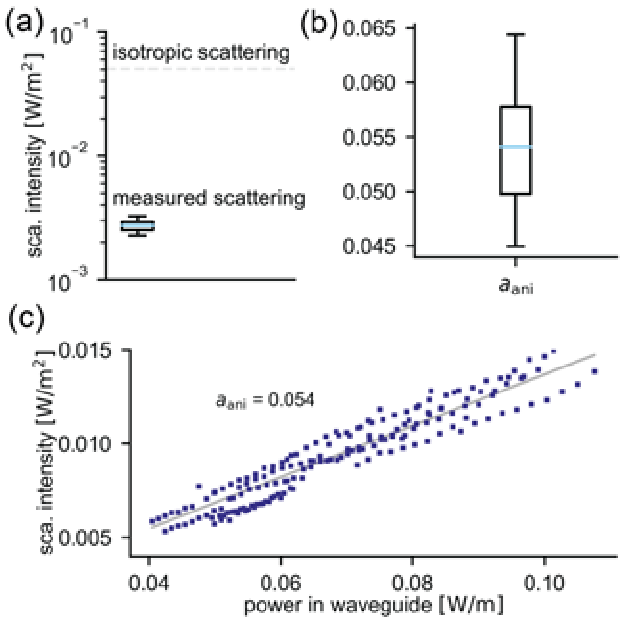


FIG. 19: Anisotropic scattering coefficient $a_{\mathrm{ani}}$(a) Measured scattered intensity with a 0.4 NA objective 100 µm away from the surface on the substrate side compared to isotropic scattering. The intensity is independent of the distance. Individual damping constants were normalized to a damping of 2.51 dB/cm [Fig. 18]. Power in the waveguide was normalized to a value of 0.02 W/m. Box plots are based on 180 measurements of image size 280 x 210 µm with 110 nm pixel size of three different chips. (b) $a_{\mathrm{ani}}$ for the investigated waveguide configuration. The median of the coefficient amounted to 0.054. (c) Intensity measured as a function of the power in the waveguide. The grey line is a least squares fit through the data and as expected yields the same value for the anisotropic scattering coefficient.

Barbara]. The microscope was operated with Bruker Nanoscope V 9.1. Height images were recorded under tapping mode operation using etched silicon cantilevers with a nominal spring constant of k = 20-80 N/m [Bruker AFM Probes, RTESPA]. An image area of 20 x 20 µm$^2$ was scanned with a resolution of 5210 x 256 pixels, and at limited z-scanner range of < 1 µm. The slow scanning axis [5210] was oriented perpendicular to the chip main axis. Height raw data were tilt-corrected followed by plane correction using a 2$^{\mathrm{nd}}$ order polynomial fit [Nanoscope Analysis V1.8 R2]. A root mean square roughness of 0.6 nm was measured. The one dimensional autocorrelation function was calculated from the profile in x-direction on each line. The average autocorrelation function of all lines was taken and normalized. Due to the convolution with the tip roughness the autocorrelation function exhibited a dominant exponential decay at extremely short length scales of 10 nm [Fig. 20(b)]. Since this roughness length scale is attributed to the tip and not the surface, the autocorrelation function is plotted from 50 to 3000 nm [Fig. 20(c)]. Several superimposing exponential decays at different length scales are visible. Therefore, using the power spectral density function [PSD] instead of fitting an exponential decay to the autocorrelation function would be more appropriate. However, this leads to a less intuitive model. The exponential decay with the shortest correlation length of Fig. 20(c) was extrapolated to 0 [Fig. 20(d)]. Then the extrapolated first 50 nm were concatenated with the autocorrelation from 50 nm to 20000 nm. The normalized autocorrelation function and an exponentially decaying fit are shown in Fig. 20(d). The fit results in a correlation length of 588 nm.

### F. Influence of waveguide parameters on signal and background

Waveguide parameters such as the refractive indices $n_{\mathrm{f}}$, $n_{\mathrm{c}}$, $n_{\mathrm{s}}$, the thickness $t_{\mathrm{f}}$ or the wavelength have a significant influence on signal and background intensities. Therefore, we explain some dependencies in this section. The intensity of the signal scales with the intensity of the electromagnetic field at the film/cover interface [see Fig. 21(a)]. This is closely related to the sensitivity of the waveguide to ad-layer changes as described in Ref. [23]. However, while the sensitivity to ad-layer changes accounts for the entire evanescent field, the molographic signal [in the configuration of this manuscript] stems from the surface only. It should be pointed out that scattering at non-specifically adsorbed molecules scales in the same fashion with respect to the waveguide parameters as the signal. The reason for this is that the scatterers have the same index contrast and that they are also located on the waveguide surface. Scattering at the surface roughness has a similar behavior with two exceptions [see Fig. 21(b)]. First of all, both interfaces need to be considered and it is affected by the optical contrast at the interfaces. Hence, a lower film refractive index increases the signal to surface scattering ratio, although the signal itself decreases for a lower refractive index [see Fig. 21(d)]. In order to make a fair comparison between waveguides of different refractive indices, the thickness of the waveguide was adapted such that the ratio of the intensity at the respective thickness to the maximum intensity for the chosen refractive index was kept constant [see Fig. 21(a): The ratio of the maximum of the dark blue curve to the sensitivity at the intersection of the dashed green line (ii) and the dark blue curve is kept constant for any refractive index]. When calculating the FOM with a theoretical estimation of the background the absolute values must be seen as approximations. However, the formula can identify the dependency of the FOM with respect to different parameters. Yet, it must be noted that Fig. 21(d) neglects any volume scattering which might become dominant for thicker waveguides. The scattering at inhomogeneities inside the waveguide on the other hand depends on the power inside the waveguide. It scales in the opposite fashion with respect to the film thickness as

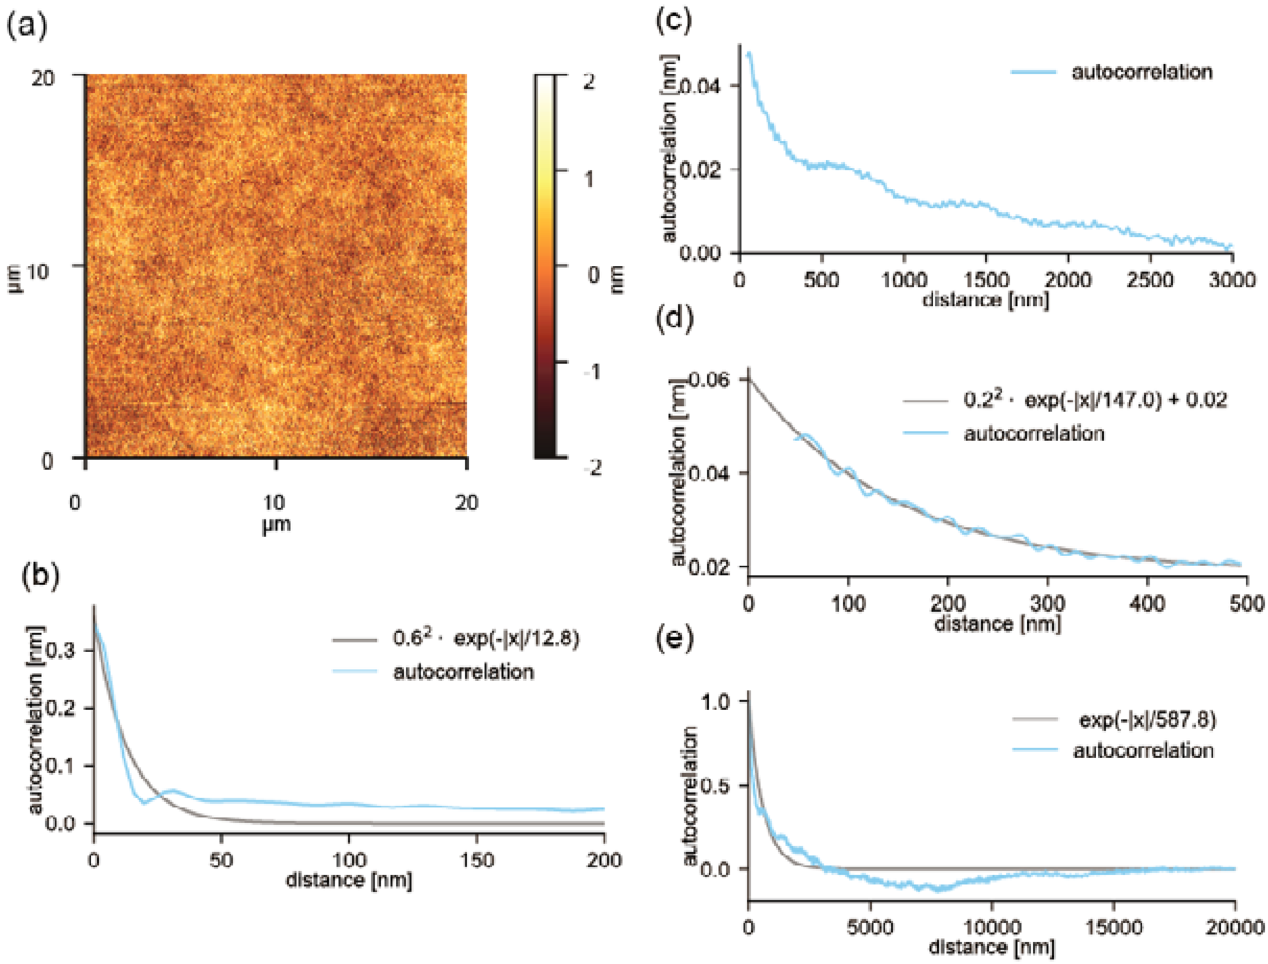


FIG. 20: Waveguide surface roughness characterization (a) Atomic force microscopy image of the waveguide surface (b) The average autocorrelation function of the surface roughness in x-direction normalized to its length is shown. An exponential fit suggests a correlation length of 12.8 nm. Yet, this is an artefact due to the convolution of the roughness with the AFM tip. (c) The autocorrelation function is therefore plotted from 50 to 3000 nm without the contribution from the tip. Several superimposed exponential decays are visible. (d) To obtain the missing data points that were lost due to the convolution with the tip, an extrapolation for the first 50 nm was performed with the exponential fit to the first decay [50 - 500 nm]. (e) The extrapolation is concatenated with the normalized autocorrelation function from 50 to 20000 nm and an exponential fit is performed to extract the correlation length of the surface roughness of 588 nm.

the intensity on the surface [see Fig. 21(c)]. The power inside the waveguide film is basically independent on the refractive index of the waveguide, when the thickness is adapted in the same way as described above [see Fig. 21(e)]. However, this cannot be directly transferred to the volume scattering, since the refractive index inhomogeneities inside the volume depend on the refractive index of the film.

### G. Noise estimation and speckle statistics

#### 1. *Estimation of* $\frac{I_{sig}}{I_{bg}}$ *for endpoint measurements*

In an endpoint measurement the variance of the ratio of the maximum pixel to the mean of different images is the relevant quantity. Fig. 22 shows the variation of the mean and the maximum pixel of the image for 180 images, as well as the variation of their ratio. The maximum pixel is 8.1 [median is with 95 % confidence between 7.9 and 8.3] times higher than the measured mean of the background intensity due to waveguide surface roughness scattering. The 99.5 % quantile of the ratio maximum/mean background that allows to estimate the detection limit in an endpoint measurement

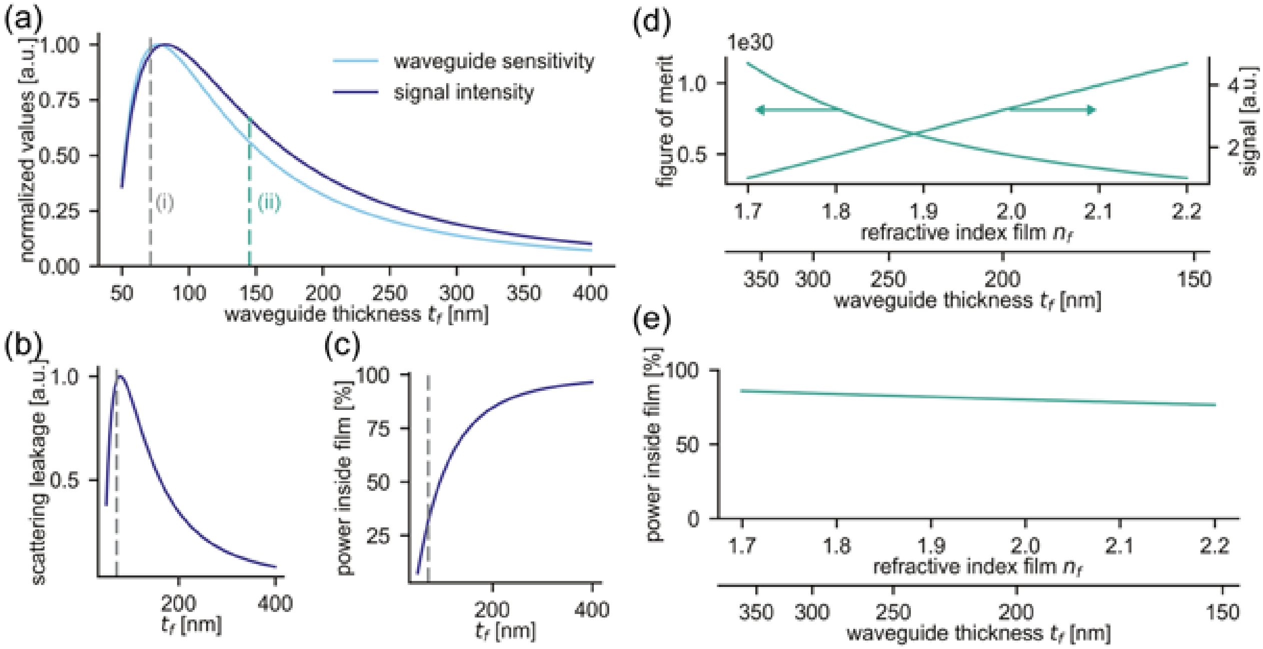


FIG. 21: (a) normalized signal intensity [which corresponds to the intensity on the surface] and waveguide sensitivity to ad-layer changes as a function of waveguide thickness for a $Ta_2O_5$ waveguide. The dashed gray line (i) indicates the cutoff thickness. The dashed green line (ii) indicates the thickness for the waveguides used in this paper. (b) surface scattering leakage against waveguide thickness (c) power inside the waveguide film against waveguide thickness (d) calculated figure of merit [neglecting any volume scattering] against the waveguide index [for $L_c$ = 588 nm, $\sigma$ = 0.6 nm and NA = 0.4]. The waveguide thickness was adapted with respect to the refractive index to enable a fair comparison between different indices. The ratio of the signal intensity at the respective waveguide thickness to the maximal possible intensity for the chosen respective refractive index was kept constant. On the second y-axis the dependency of the signal to the refractive index is illustrated. It should be noted that using the formula for the scattering results in an approximation of the FOM and not exact values (e) Power inside the waveguide against the refractive index of the film. The thickness was adapted as described in (c). For the calculations of the curves the following waveguide parameters were used: $n_c = 1$, $n_s = 1.521$, $\lambda = 632.8$ nm for (a), (b) and (c) $n_f = 2.117$

with the specified field of view is 13.8. If the position of the molographic spot can be constrained to a smaller field of view, this ratio decreases. In the limit when the position of the molographic spot is precisely known it reduces to the the expected variation of a single speckle determined by speckle statistics [24]. Fig. 23 shows the histogram of the speckle intensities before (a) and after a convolution operation with the Airy disk of the mologram (b). Before convolution, the distribution of the measured intensities follows a nearly perfect negative exponential distribution [24] and the ratio of the 99.7 percentile and mean is close to the expected value from the negative exponential distribution $\frac{q_{99.7}}{\mu} = -\ln(0.003) = 5.8$. After convolution, the speckle statistics deviates from the exponential distribution, rendered more gaussian [24], and the median of the ratio of the 99.7 percentile and mean is 3.33. Therefore, the precise knowledge of the molographic spot would only give a slightly better detection limit of 1.5 pg/mm$^2$ in endpoint measurements.

### 2. Influence of large background scatterers

*a. In terms of total power* To investigate the importance of large background scatterers, we acquired 20 images of the surface of one cleaned chip [30s $O_2$ plasma followed by 10 min sonication in DI water]. Images were thresholded [15 times the mean of the image] and everything above this was taken as power that originated from large scatterers. Fig. 24 shows that below 1 % of the total power leaving the waveguide is due to large scattering centers. Therefore, in terms of total power this background contribution is negligible for properly cleaned chips.

*b. As a function of distance* Despite the overall power scattered being small, a large particle on the waveguide surface will cause an inhomogeneous background that may interfere with the molographic measurement. Molographic foci should therefore be sufficiently distant to the waveguide surface. To obtain a rough estimate of this distance, we acquired images of the scattered field at various positions from the waveguide at a location where there was substantial particle contamination and calculated the value of the maximum pixel and the mean of the image [Fig. 24]. One can see that the in-

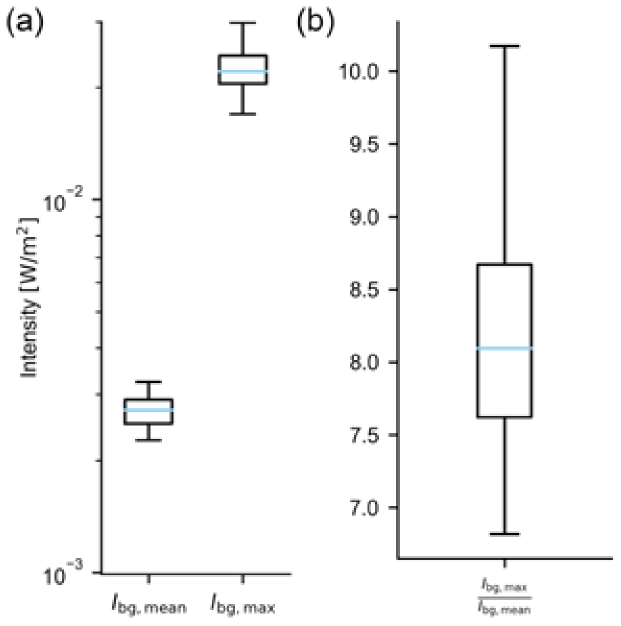


FIG. 22: Estimation of $\frac{I_{\rm sig}}{I_{\rm bg}}$ for endpoint measurements (a) Mean and maximum of the background intensity in the focal plane after convoluting the images with an Airy function of the numerical aperture of the objective [NA = 0.4], which is equivalent of trying to detect a molographic spot from a mologram with NA = 0.4. (b) Ratio of maximum background intensity [maximum pixel] and mean background in the focal plane. Box plots are based on 180 measurements of image size 280 x 210 µm with 110 nm pixel size of three different chips and were convoluted with the expected Airy disk of the mologram.

fluence becomes negligible beyond 80 - 100 µm from the waveguide surface for an 0.4 NA objective and a scattering leakage of roughly 6 /m. The exact distance will be a function of the scatterer size and refractive index, the penetration depth of the evanescent field, the numerical aperture of the optics and the intensity of the waveguide background. The precise derivation of this expression is beyond the scope of this publication, but as a rule of thumb, for a given scatterer size, the distance is inversely proportional to the numerical aperture of the mologram and the square root of the scattering leakage.

$$f \propto \frac{1}{\rm NA}\frac{1}{\sqrt{a_{\rm ani}\alpha_{\rm sca}}} \qquad (76)$$

To give an example, for a numerical aperture of 0.1 and a scattering leakage of 0.6 /m, the focal plane should be roughly an order of magnitude further away than in our case [distance always in air].

## IX. RESOLUTION OF FOCAL MOLOGRAPHY AND COMPARISON TO SPR

### A. Choice of the reference intensity for focal molography

It is not straightforward to choose the intensity reference in focal molography. One option would be to split the input beam and use this as the reference. Yet, this is not particularly useful since variations in the in-coupling efficiency would not be compensated. Also measuring the power in the waveguide via the out-coupling grating during a measurement will lead to drifts, since any change in scattering over the entire propagation distance will affect the remaining power at the out-coupling grating. The most suitable intensity reference is therefore the waveguide background or a reference spot in the focal plane, since the majority of fluctuations will affect it in exactly the same way as the molographic focus. Here we chose the waveguide background and provide the formulas for this reference.

### B. Derivation of the limit of detection formula for focal molography

The mass density on the mologram can be computed from the average intensity in the Airy disk by starting from

$$\begin{aligned} I_{\rm avg,RS} &= 2.536\cdot\pi^2\frac{{A_{\rm mologram}}^2}{{A_+}^2}{\rm NA}^2 n_{\rm c}^2\frac{\left(n_{\rm P}^2-n_{\rm c}^2\right)^2}{\left(n_{\rm P}^2+2n_{\rm c}^2\right)^2} \\ &\times\frac{D^2}{\lambda^4}\frac{{\eta_{\rm mod[A]}}^2\Gamma^2}{\rho_{\rm P}^2}\frac{n_c\left(n_{\rm f}^2-N^2\right)}{Nt_{\rm eff}\left(n_{\rm f}^2-n_{\rm c}^2\right)}P_{\rm wg} \qquad (77)\end{aligned}$$

It is advantageous to use a different algorithm to compute the molographic signal and adapting this expression to the standard readout algorithm of the convolution with the normalized Airy disk kernel [see SM Section X C].

$$\frac{I_{\rm sig}}{I_{\rm Airy,max}} = \left.\left(\frac{2J_1\left(r\right)}{r}\right)^2 * \frac{\left(\frac{2J_1(r)}{r}\right)^2}{\int\limits_0^{2\pi}\int\limits_0^{\infty}\left(\frac{2J_1(r)}{r}\right)^2 r dr}\right|_{r=0} = 0.4596 \qquad (78)$$

Hence, from Eqs. (40) and (78) it follows that $I_{\rm sig} = 2.012\cdot I_{\rm avg}$. Inserting this into Eq. (77) and rearranging to

$$\begin{aligned}\Gamma &= \frac{A_+}{A_{\rm mologram}}\frac{1}{\eta_{\rm mod[A]}}\frac{\lambda^2}{D}\frac{\rho_{\rm P}\left(n_{\rm P}^2+2n_{\rm c}^2\right)}{n_{\rm c}\left(n_{\rm P}^2-n_{\rm c}^2\right)} \\ &\times\sqrt{\frac{I_{\rm sig}}{5.102\cdot\pi^2{\rm NA}^2\frac{n_c\left(n_{\rm f}^2-N^2\right)}{Nt_{\rm eff}\left(n_{\rm f}^2-n_{\rm c}^2\right)}P_{\rm wg}}} \qquad (79)\end{aligned}$$

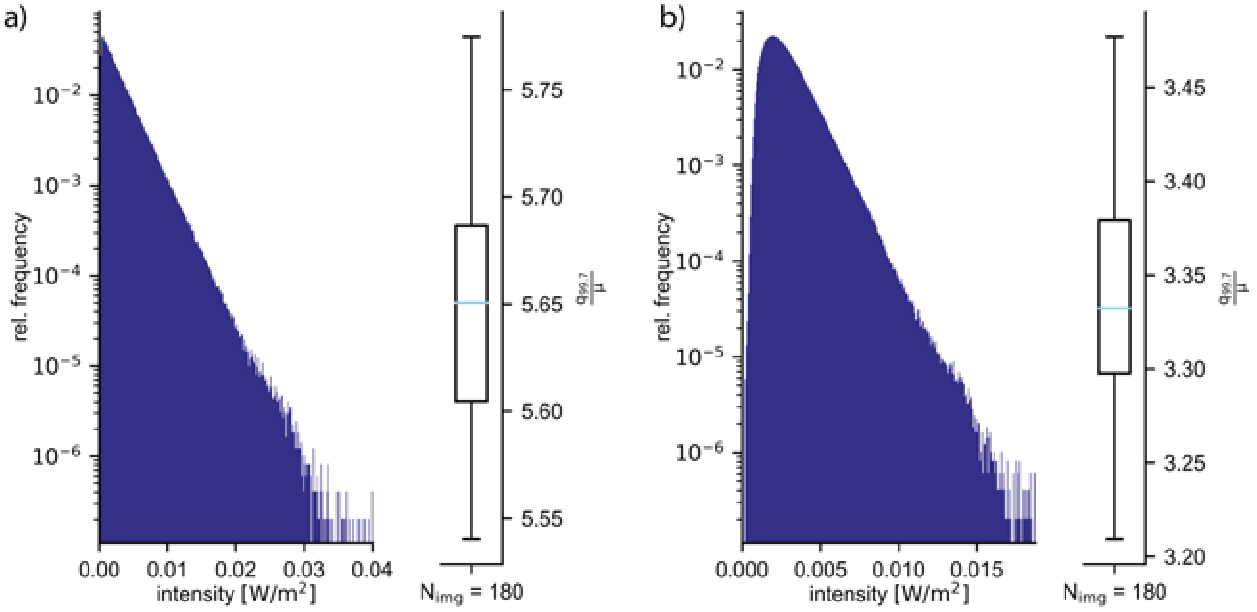


FIG. 23: Distribution of speckle intensities and distribution of the 99.7 percentile divided by the mean. (a) before convolution with the Airy disk and (b) after convolution with the Airy disk of the mologram (NA = 0.4). The speckle intensities have been normalized to a power per unit length in the waveguide of 0.02 W/m.

The power in the waveguide can then be expressed from the average intensity of the background according to Eq. (5): $P_{\text{wg}} = \frac{4I_{\text{bg}}}{a_{\text{ani}}\alpha_{\text{sca}}\text{NA}^2}$, which yields

$$\Gamma = 0.0704 \cdot \frac{A_+}{A_{\text{mologram}}} \frac{1}{\eta_{\text{mod[A]}}} \sqrt{\frac{a_{\text{ani}}\alpha_{\text{sca}}}{\frac{n_c\left(n_f^2-N^2\right)}{Nt_{\text{eff}}\left(n_f^2-n_c^2\right)}}} \times \frac{\lambda^2}{D} \frac{\rho_{\text{P}}\left(n_{\text{P}}^2+2n_c^2\right)}{n_c\left(n_{\text{P}}^2-n_c^2\right)} \sqrt{\frac{I_{\text{sig}}}{I_{\text{bg}}}} \tag{80}$$

This can also be written in terms of the refractive index increment for proteins.

$$\Gamma = 0.1056 \cdot \frac{A_+}{A_{\text{mologram}}} \frac{1}{\eta_{\text{mod[A]}}} \frac{1}{\frac{dn}{dc}} \sqrt{\frac{a_{\text{ani}}\alpha_{\text{sca}}}{\frac{n_c\left(n_f^2-N^2\right)}{Nt_{\text{eff}}\left(n_f^2-n_c^2\right)}}} \times \frac{\lambda^2}{D} \sqrt{\frac{I_{\text{sig}}}{I_{\text{bg}}}} \tag{81}$$

from which $\Gamma_0$ can be identified

$$\Gamma_0 = 0.1056 \cdot \frac{A_+}{A_{\text{mologram}}} \frac{1}{\eta_{\text{mod[A]}}} \times \sqrt{\frac{a_{\text{ani}}\alpha_{\text{sca}}}{\frac{n_c\left(n_f^2-N^2\right)}{Nt_{\text{eff}}\left(n_f^2-n_c^2\right)}}} \frac{\lambda^2}{D\frac{dn}{dc}} \tag{82}$$

## C. Derivation of the sensitivity of SPR

The aim of this section is to derive the sensitivity of SPR, which links the RMS noise of the relative intensity [reflectance changes] to the RMS noise of the ad-layer mass density changes. It has to be noted that the reflectivity is normalized to the input beam power. However, since the reflectivity in intensity interrogation mode [at the location of maximum slope] is usually $R = 0.5$ [25], therefore this equation is still a good estimate of the required precision of the intensity measurement at the detector.

$$\text{RMS}_{R-\langle R\rangle} = S_\Gamma \text{RMS}_{\Gamma-\langle\Gamma\rangle} \tag{83}$$

or in terms of effective refractive index

$$\text{RMS}_{R-\langle R\rangle} = S_N \text{RMS}_{N-\langle N\rangle} \tag{84}$$

respectively. The sensitivities are defined by

$$S_N = \frac{\partial R}{\partial N} \qquad S_\Gamma = \frac{\partial R}{\partial \Gamma} \tag{85}$$

$\text{RMS}_{R-\langle R\rangle}$, $\text{RMS}_{N-\langle N\rangle}$ and $\text{RMS}_{\Gamma-\langle\Gamma\rangle}$ are root mean square noise of the reflectivity, the effective refractive index and surface mass density, respectively.

We first aim to find an expression for the effective refractive index sensitivity $S_N$. From [26] we know that the maximum change in reflectivity of the SPR signal is given by

$$\left(\frac{dR}{dk_x}\right)_{\max} = 3\frac{\sqrt{3}}{2}\frac{\gamma_i\gamma_r}{\left(\gamma_i+\gamma_r\right)^3} \tag{86}$$

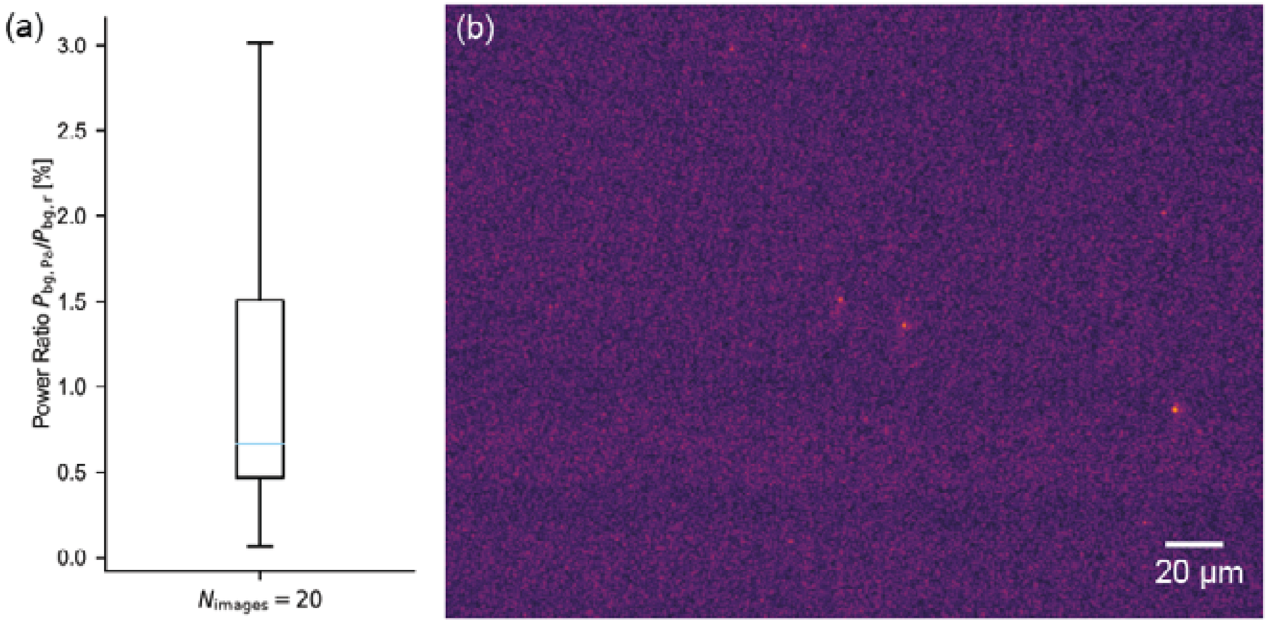


FIG. 24: relative importance of the power scattered by large dust particles relative to power scattered from waveguide sidewall roughness (a) box plot of the power ratio $\frac{P_{\mathrm{bg,r}}}{P_{\mathrm{bg,Pa}}}$, median is 0.66 % with 95 % confidence in interval [0.47, 1.47] (b) typical waveguide surface image with a few dust particles. The power norm chosen for plotting [inferno color map] is 0.25 in order to better visualize the waveguide background.

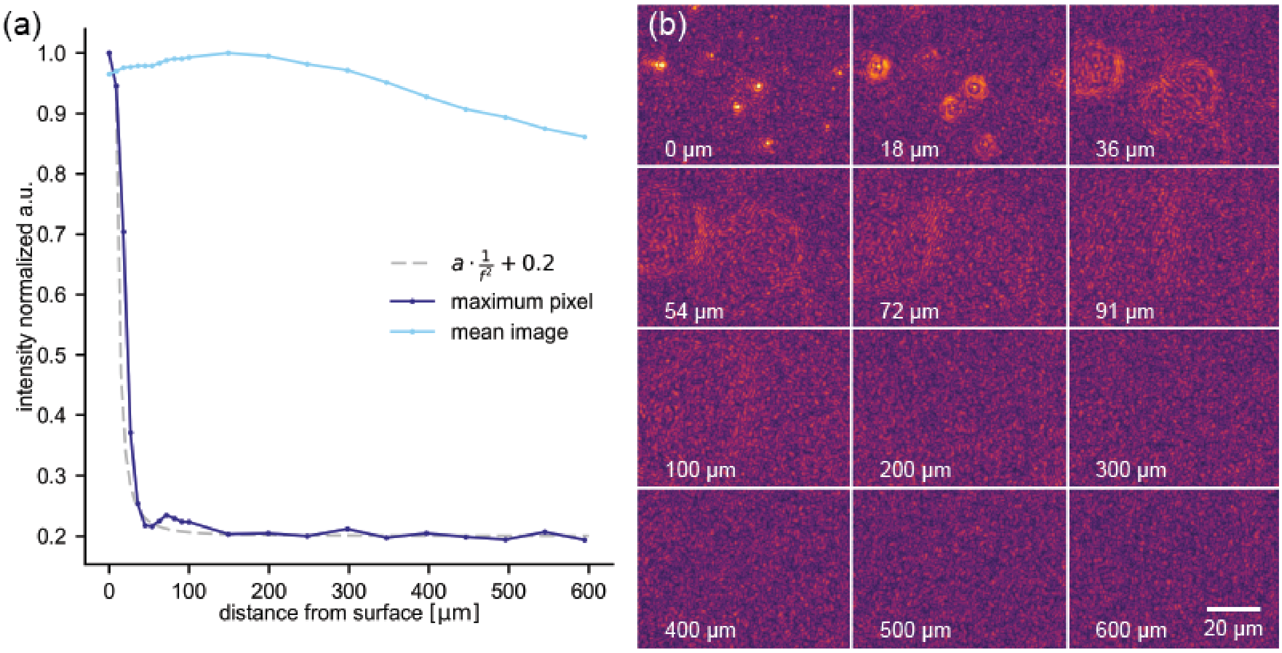


FIG. 25: relative importance of large scatterer centers for the homogeneity of the speckle background. (a) maximum pixel and mean of the image normalized to the value at the surface calculated from seven approach curves. Images were acquired by a 0.4 NA objective. The mean is nearly independent of distance as expected from the expression of the waveguide background intensity for a constant aperture. The decrease for larger distances is due to the finite beam width of 1 mm. The maximum pixel first decreases with a reciprocal quadratic relationship and then approaches the waveguide background [dashed line] the function is normalized to the datapoint closest to the waveguide surface [9 μm]. (b) exemplary images highlighting the decrease of importance of large scatterers with increasing distance from the waveguide.

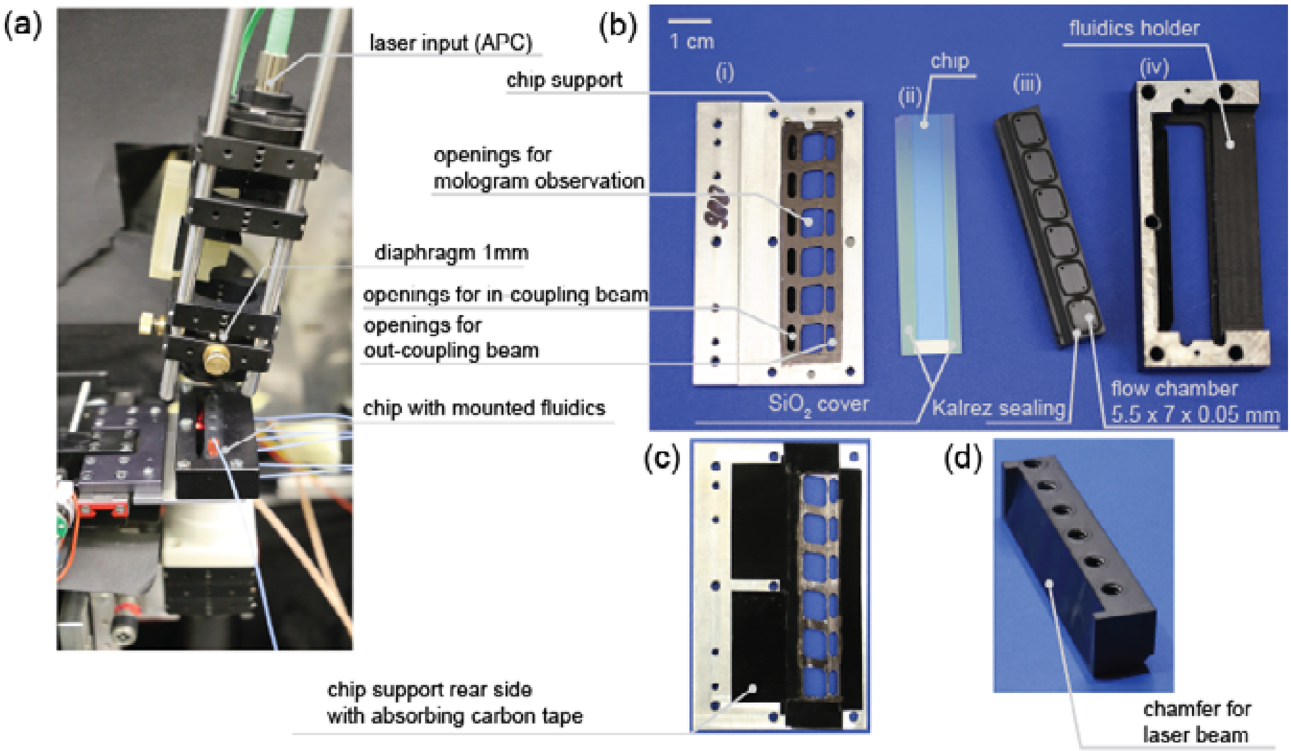


FIG. 26: MoloReader configuration for real time measurements. (a) chip with mounted fluidics, connectors used were F-126-H [Ercatech AG] for 1/32" tubing [FEP009-031-B 225 µm internal diameter]. (b) the chip fluidics assembly disassembled. From left to right: An aluminium chip holder (i) was machined with openings for in-coupling and out-coupling beams as well as for observation with the microscope. It is important that the sealing is supported everywhere with aluminium otherwise the chip breaks upon tightening the screws. The rear side of the holder is shown in (c), straylight was reduced at all important locations by means of a black waterproof pen or MetalVelvet$^{TM}$ Adhesive [ACM Coatings]. The waveguide chips (ii) [IMT Masken und Teilungen AG, Greifensee, Switzerland] were described in the main text, for the real-time measurements the coupling gratings were covered with $SiO_2$ [ca. 1 µm] in order to avoid damping of the mode at the black Kalrez flat packing [laser cutted from a sheet of Kalrez 0.5 mm thickness]. Each flow chamber has a volume of roughly 2 µl. (iii) PEEK fluidics housing in bottom view [front view in (d)] six fluidic chambers are individually addressable (iv) aluminium holder for the PEEK fluidic body. (d) The PEEK body has a chamfer with - 12° angle for the laser beam to reach the coupling grating.

$k_x$ is the in plane wavevector. $\gamma_\mathrm{i}$ is the intrinsic damping of the plasmon and $\gamma_\mathrm{r}$ is the radiation damping. The sensitivity is maximized when $\gamma_\mathrm{r} = \frac{\gamma_\mathrm{i}}{2}$. This is different from the perfectly matched case $\gamma_\mathrm{r} = \gamma_\mathrm{i}$ when the reflectivity is zero, which can be explained that although the reflectivity at resonance is not zero, the slope is maximized. Inserting this into Eq. (86) yields

$$\frac{dR}{dk_\mathrm{x}} = \frac{2\sqrt{3}}{9\gamma_\mathrm{i}} \tag{87}$$

The intrinsic damping of the film is

$$\gamma_\mathrm{i} = \frac{{n_\mathrm{c}}^3 k_0 \varepsilon_\mathrm{i}}{2{\varepsilon_\mathrm{r}}^2} \tag{88}$$

whereas $\varepsilon_\mathrm{r}$ and $\varepsilon_\mathrm{i}$ are real and imaginary part of the permittivity of the metal, respectively. By using $k_x = N \cdot k_0$ and $\frac{dk_x}{dN} = k_0$ , we can find for $S_N$

$$S_N = \frac{dR}{dN} = \frac{dR}{dk_x}\frac{dk_x}{dN} \approx \frac{dR}{dk_x}k_0 = \frac{2\sqrt{3}}{9\gamma_\mathrm{i}}k_0 \tag{89}$$

Inserting the expression for the damping constant [Chapter 4.1 in [27]] we obtain for the sensitivity with respect to effective index changes.

$$S_N = \frac{4\sqrt{3}{\varepsilon_\mathrm{r}}^2}{9{n_\mathrm{c}}^3\varepsilon_\mathrm{i}} \tag{90}$$

This expression is maximized, when the damping of the SPR film is minimized. The minimum damping of a gold film is reached at 700 nm with a permittivity of $\varepsilon = -16 + i1.1$ [28]. For gold at 700 nm the sensitivity for refractive index changes is roughly 76. Hence, in order to resolve a refractive index change of $\Delta N = 10^{-7}$ as in the best SPR measurements reported [28] one needs measure the intensity with a precision of roughly $10^{-5}$ or 0.001% reflectivity change.

Lastly, we need to derive the sensitivity in terms of surface mass density. The sensitivity of the effective refractive index as a function of surface mass density was derived by Lukosz [16].

$$\Delta N = \frac{4\pi N^4}{\lambda(-\varepsilon_r)^{\frac{1}{2}}} \frac{1}{{n_c}^2} \frac{dn}{dc} \Delta\Gamma \tag{91}$$

With this expression and noting that in Eq. (88) one should correctly use the effective index [29], we obtain the sensitivity equation of SPR with respect to surface mass changes for intensity interrogation.

$$S_\Gamma = \frac{\partial R}{\partial \Gamma} = \frac{16\sqrt{3}{\varepsilon_\mathrm{r}}^2}{9\varepsilon_\mathrm{i}(-\varepsilon_r)^{\frac{1}{2}}} \frac{\pi N}{\lambda n_\mathrm{c}^2} \frac{dn}{dc} \tag{92}$$

Inserting the values for gold at 700 nm and using the calculated effective index of 1.41 one obtains $S_\Gamma = 1.16 \cdot 10^5[\mathrm{mm}^2/\mathrm{pg}]$.

### D. Derivation of the sensitivity of focal molography

The sensitivity of focal molography can be derived accordingly. The intensity reference in molography is not the input power that hits the grating coupler but rather the intensity of the average background in the focal plane. We start from

$$\begin{aligned} \frac{I_\mathrm{sig}}{I_\mathrm{bg}} &= 89.4 \cdot \frac{{A_\mathrm{mologram}}^2}{{A_+}^2} \left(\frac{dn}{dc}\right)^2 \frac{D^2}{\lambda^4} \\ &\times {\eta_\mathrm{mod[A]}}^2 \frac{n_c\left(n_\mathrm{f}^2 - N^2\right)}{N t_\mathrm{eff}\left(n_\mathrm{f}^2 - n_\mathrm{c}^2\right)} \frac{1}{a_\mathrm{ani}\alpha_\mathrm{sca}} \Gamma^2 \end{aligned} \tag{93}$$

where we have replaced the power in the waveguide $P_\mathrm{wg}$ by the average background intensity. This is a relative intensity in exactly the same way as the reflectivity in SPR. We take the derivative with respect to molographic surface mass density to obtain the sensitivity equation.

$$\begin{aligned} S_\Gamma &= \frac{\partial \frac{I_\mathrm{sig}}{I_\mathrm{bg}}}{\partial \Gamma} = 178.8 \cdot \frac{{A_\mathrm{mologram}}^2}{{A_+}^2} \left(\frac{dn}{dc}\right)^2 \frac{D^2}{\lambda^4} \\ &\times {\eta_\mathrm{mod[A]}}^2 \frac{n_c\left(n_\mathrm{f}^2 - N^2\right)}{N t_\mathrm{eff}\left(n_\mathrm{f}^2 - n_\mathrm{c}^2\right)} \frac{1}{a_\mathrm{ani}\alpha_\mathrm{sca}} \Gamma \\ &= \frac{2}{{\Gamma_0}^2}\Gamma \end{aligned} \tag{94}$$

By assuming that the operation point is close to the background intensity $[\Gamma = \Gamma_0]$, which is a valid approximation, the sensitivity of focal molography reads.

$$\begin{aligned} S_{\Gamma_\mathrm{FM}} &= \frac{\partial \frac{I_\mathrm{sig}}{I_\mathrm{bg}}}{\partial \Gamma} \\ &= 18.9 \cdot \frac{A_\mathrm{mologram}\eta_\mathrm{mod[A]}}{A_+} \frac{dn}{dc} \\ &\times \frac{D}{\lambda^2} \sqrt{\frac{n_c\left(n_\mathrm{f}^2 - N^2\right)}{N t_\mathrm{eff}\left(n_\mathrm{f}^2 - n_\mathrm{c}^2\right) a_\mathrm{ani}\alpha_\mathrm{sca}}} \\ &= \frac{2}{\Gamma_0} \propto \sqrt{\mathrm{FOM_{FM}}} \end{aligned} \tag{95}$$

Alternatively, the sensitivity can be derived from $\Gamma = \Gamma_0\sqrt{\frac{I_\mathrm{sig}}{I_\mathrm{bg}}}$. By writing $I_\mathrm{sig} = I_\mathrm{bg} + \Delta I$ and performing a Taylor expansion up to first order one obtains.

$$\Gamma - \Gamma_0 = \frac{\Gamma_0}{2} \frac{\Delta I}{I_\mathrm{bg}} \tag{96}$$

From the definition $\frac{I_\mathrm{sig}}{I_\mathrm{bg}} - \left\langle \frac{I_\mathrm{sig}}{I_\mathrm{bg}} \right\rangle = \frac{\Delta I}{I_\mathrm{bg}}$ and again assuming that the operating point is close to the background intensity $[\Gamma_0 = \langle\Gamma\rangle]$ it follows that the RMS values of intensity and molographic surface mass density are connected accordingly.

$$\mathrm{RMS}_{\frac{I_\mathrm{sig}}{I_\mathrm{bg}} - \left\langle \frac{I_\mathrm{sig}}{I_\mathrm{bg}} \right\rangle} = \frac{2}{\Gamma_0} \mathrm{RMS}_{\Gamma - \langle\Gamma\rangle} \tag{97}$$

The factor 2 stems from the quadratic sensor transfer function. Inserting the FOM of molography used in the real-time measurements, one obtains a sensitivity of $S_\Gamma = 1.1 \cdot 10^9\ [\mathrm{mm}^2/\mathrm{pg}]$. Thanks to this much higher sensitivity, molography can achieve the same resolution as SPR with much larger intensity noise. The sensitivity is therefore not suitable to compare the two techniques, since its value depends on the chosen intensity reference.

## X. REAL-TIME MEASUREMENTS

### A. Instrumentation for real time measurements

For the real-time measurements a flow cell and chips with $SiO_2$ covered coupling gratings were developed. Fig. 26(a) shows the reader with the mounted flow cell. Fig. 26(b)-(d) display the unmounted flow cell assembly. The design of the flow chamber was similar as in our last publication [5]. However, there is one significant difference between the MoloReader and the ZeptoReader. The MoloReader couples in from the top and outside the flow chamber [compared to the bottom coupling of the ZeptoReader] and therefore at one point the guided mode needs to cross the sealing of the flow chamber. Here we would like to emphasize that designing a fluidics for a waveguide where the mode has to cross the sealing is not

straightforward at all. To our knowledge, the only solution is to encapsulate the evanescent part of the field in a silica coating where the mode crosses the sealing. Without any protective $SiO_2$ cover any opaque sealing material [like Kalrez] completely extincts the mode. Transparent materials such as PDMS are also unsuitable since they act as lenses that alter the wavefront of the coupled mode. This leads to a sickle-like deformation of the focal spot, changing with the pressure in the flow chamber.

### B. Localization of molographic foci for real-time measurements

The focal plane is determined by the numerical aperture of the mologram and can be easily found by knowing the location of the surface. More challenging in our experimental setting was to have the Airy disk in the field of view. To accomplish this, biotin molograms [NH-biotin|$NH_2$] were fabricated as described in the main manuscript. Then HBS-T buffer was manually injected and the position of the now weaker focal spot was precisely determined in the speckle pattern. Subsequently, the grooves were backfilled by manually injecting 500 µl of 5 mM NHS-PEG$_{12}$-OMe in HBS-T buffer for 15 min and then rinsed with PBS-T. The backfilling resulted in the focal spot to disappear in the speckle pattern.

### C. Processing of real-time binding signals

The processing of real-time signals was carried out offline. First, the images were registered in order to compensate for temperature related movements of the focal spot in the focal plane [Fig. 27(a)]. After registration, the images were convoluted with the shape of the Airy disk to obtain a weighted averaging over the Airy disk to decrease the influence of hot pixels and pixel noise [Fig. 27(b)]. Each pixel in the convoluted image is related to the average intensity in the Airy disk surrounding it by $I_{\mathrm{sig}} = 2.012 \cdot I_{\mathrm{avg}}$. This form of averaging is a tradeoff between taking the maximum pixel only [not robust to hot pixels and pixel noise] or uniformly averaging over the Airy disk [too conservative]. Subsequently, the images were segmented into signal detection region of interest [$\mathrm{ROI}_{\mathrm{sig}}$] the region of interest for normalization [$\mathrm{ROI}_{\mathrm{norm}}$] and the pixel chosen for reference binding traces Fig. 27(c)]. The signal trace was obtained from the location of the highest pixel in the signal region of the last image of the experiment [molographic signal was only visible after binding]. In general, any pixel of the convoluted image is a potential candidate for a binding trace, however they should be sufficiently distant to each other in order not to be correlated. Therefore, the reference binding traces are spaced such that their speckles do not overlap after the convolution operation and therefore the traces are non-correlated. This allows to extract more hypothetical binding traces and to characterize their noise levels [Fig. 28]. Finally, the goal is to obtain signal and reference binding traces that are normalized to the mean intensity of the first image. The first step [Fig. 27(d)] is to compute the average intensity on the $\mathrm{ROI}_{\mathrm{norm}}$ of the first image. This value is used for three different computations which are indicated by different arrows. First, the signal and reference traces are normalized by the average intensity of the first image. These normalized traces still contain the drift of the power in the waveguide [due to coupling efficiency changes]. By normalizing the average intensity of each image on the $\mathrm{ROI}_{\mathrm{norm}}$ to the value of the first image [Fig. 27(e)] and multiplying this with the normalized traces one obtains the drift compensated relative intensity curves with respect to the average waveguide background of the first image [see Fig. 27(f)]. The reason for this rather complicated referencing procedure becomes apparent from the third use of the average intensity on the $\mathrm{ROI}_{\mathrm{norm}}$ of the first image. Because the scattering leakage of the waveguide was measured, we can get the initial waveguide power $P_{\mathrm{wg,ini}}$ and calculate the equivalent molographic mass density that would correspond to this intensity and then multiply it with the square root of the drift compensated relative intensity curves. This finally yields the molographic mass binding traces [Fig. 27(g)]. We can only do this operation because they are all normalized to the average intensity in the first image and the equivalent coherent mass density $\Gamma_0$ was calculated form this value. From these curves one can then subtract the baseline and plot the final intensity and binding curves that were used to calculate the RMS values of intensity and molographic mass density [Fig. 27(h)].

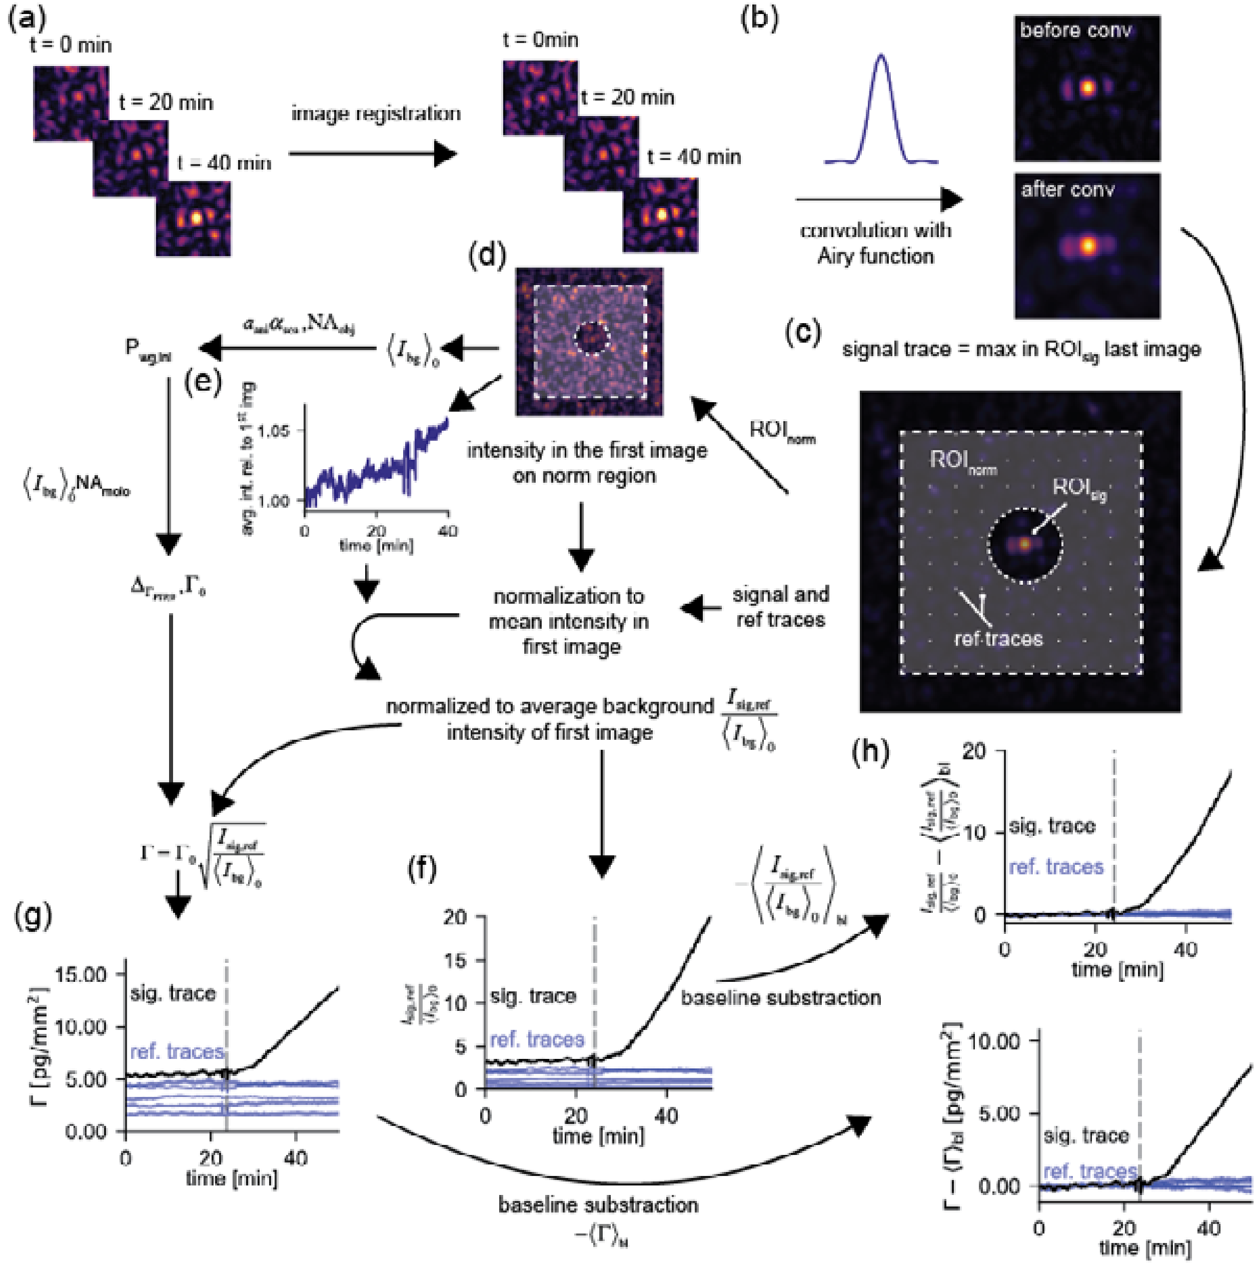


FIG. 27: Processing of the realtime binding signals. (a) Raw images were registered with TurboReg [30] to compensate for the mostly temperature induced lateral drift of the speckles in the focal plane. (b) Images were convoluted with the Airy disk of the mologram in order to decrease the influence of hot pixels and pixel noise. (c) The region of interest for normalization [$\mathrm{ROI}_{\mathrm{norm}}$], signal detection [$\mathrm{ROI}_{\mathrm{sig}}$] and the pixel chosen for reference binding traces are highlighted. The signal trace was determined from the location of the highest pixel in the last image of the binding experiment. A border of 50 pixels was discarded for the analysis due to shifts of the image registration algorithm. (d) Intensity on the $\mathrm{ROI}_{\mathrm{norm}}$ of the first image was used to normalize the intensity of each image. (e) The intensity on the $\mathrm{ROI}_{\mathrm{norm}}$ of every image was normalized to the first image in order to compensate for drifts of the laser source. (f) The normalized intensity of the signal and five reference traces as a function of time. (g) The molographic surface mass density that is equal to the measured intensity was calculated from the first image and by multiplying this value with the square root of the normalized intensity the coherent mass density traces were obtained. (h) baseline subtracted intensity and mass binding traces

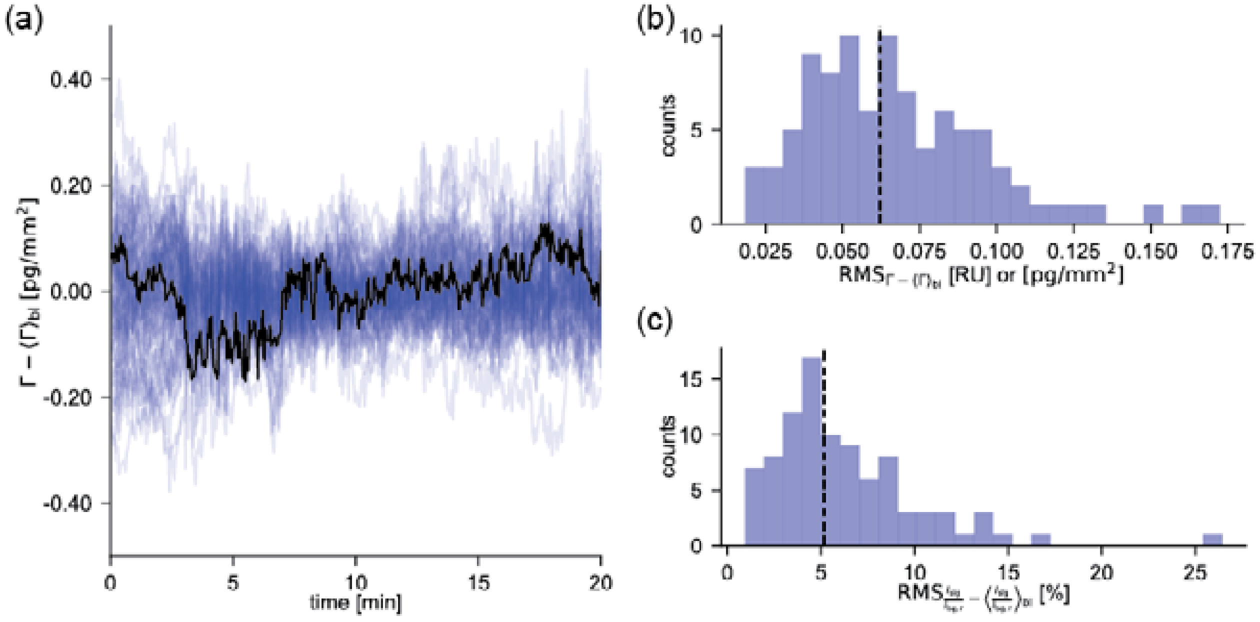


FIG. 28: Noise levels of reference traces (a) 93 reference traces from one experiment are plotted as a function time [during the 20 min baseline measurement] in units of molographic surface mass density. In black, a typical curve is highlighted. (b) histogram of the $\mathrm{RMS}_{\Gamma-\langle\Gamma\rangle_{\mathrm{bl}}}$ of the individual curves, the black dashed (–) vertical line is the median (c) histogram of the $\mathrm{RMS}_{\frac{I_{\mathrm{avg}}}{I_{\mathrm{bg,r}}}-\left\langle\frac{I_{\mathrm{avg}}}{I_{\mathrm{bg,r}}}\right\rangle_{\mathrm{bl}}}$ of the individual curves, the black dashed vertical line is the median. The RMS values were calculated from the data and not via the sensitivity of molography [Eq. (95)].


[1] R. Magnusson and T. K. Gaylord, J. Opt. Soc. Am., JOSA **68**, 806 (1978).

[2] T. M. Squires, R. J. Messinger, and S. R. Manalis, Nat. Biotechnol. **26**, 417 (2008).

[3] C. Fattinger, Phys. Rev. X **4**, 031024 (2014).

[4] T. Tamir and S. T. Peng, J. Phys. D Appl. Phys. **14**, 235 (1977).

[5] V. Gatterdam, A. Frutiger, K.-P. Stengele, D. Heindl, T. Lübbers, J. Vörös, and C. Fattinger, Nat. Nanotechnol. (2017).

[6] D. Marcuse, *Theory of dielectric optical waveguides*, Quantum electronics–principles and applications (Academic Press, 1974).

[7] D. Sinclair, J. Opt. Soc. Am. **37**, 475 (1947).

[8] T. L. McMEEKIN, M. L. Groves, and N. J. Hipp, in *Amino Acids and Serum Proteins* (AMERICAN CHEMICAL SOCIETY, 1964), vol. 44 of *Advances in Chemistry*, chap. 4, pp. 54–66.

[9] H. Zhao, P. H. Brown, and P. Schuck, Biophys. J. **100**, 2309 (2011).

[10] W. Heller, J. Phys. Chem. **69**, 1123 (1965).

[11] J. A. De Feijter, J. Benjamins, and F. A. Veer, Biopolymers **17**, 1759 (1978).

[12] H. Fischer, I. Polikarpov, and A. F. Craievich, Protein Sci. **13**, 2825 (2004).

[13] L. Novotny, J. Opt. Soc. Am. A, JOSAA **14**, 91 (1997).

[14] L. Novotny, J. Opt. Soc. Am. A, JOSAA **14**, 105 (1997).

[15] L. Novotny and B. Hecht, *Principles of Nano-Optics* (Cambridge University Press, 2011).

[16] W. Lukosz, J. Opt. Soc. Am., JOSA **71**, 744 (1981).

[17] E. Hecht, *Optics* (ADDISON WESLEY Publishing Company Incorporated, 2016).

[18] S. Martellucci and A. N. Chester, eds., *Diffractive Optics and Optical Microsystems* (1997).

[19] S. Swann, Vacuum **38**, 791 (1988).

[20] T. Nishide and F. Mizukami, Thin Solid Films **298**, 89 (1997).

[21] J. Lacey and F. P. Payne, IEE Proceedings J-Optoelectronics (1990).

[22] F. P. Payne and J. P. R. Lacey, Opt. Quantum Electron. **26**, 977 (1994).

[23] K. Tiefenthaler and W. Lukosz, J. Opt. Soc. Am. B, JOSAB **6**, 209 (1989).

[24] J. C. Dainty, in *Progress in Optics*, edited by E. Wolf (Elsevier, 1977), vol. 14, pp. 1–46.

[25] A. A. Kolomenskii, P. D. Gershon, and H. A. Schuessler, Appl. Opt. **36**, 6539 (1997).

[26] E. M. Yeatman, Biosensors and Bioelectronics **11**, 635 (1996).

[27] Homola, *Surface Plasmon Resonance Based Sensors*, vol. 4 of *Springer Series on Chemical Sensors and Biosensors* (Springer Berlin Heidelberg, Berlin, Heidelberg, 2006).

[28] M. Piliarik and J. Homola, Opt. Express **17**, 16505 (2009).

[29] W. Lukosz, Biosensors and Bioelectronics **6**, 215 (1991).

[30] P. Thévenaz, U. E. Ruttimann, and M. Unser, IEEE Trans. Image Process. **7**, 27 (1998).
